# Supplementary material for: Revisiting Chain-of-Thought Reasoning under Limited Supervision: Semi-supervised Chain-of-Thought Learning
Source: arXiv:2607.01511 source file (2026-07-01)
Supplement: Supplementary file 1 [file appendix_a.tex]

\section{Theoretical Derivation}
\label{app:proof_ib_sa}

In this section, we provide a rigorous derivation of Proposition \ref{prop:ib_sa_channel}. Let $\mathbf{X} = [\mathbf{c}_1, \dots, \mathbf{c}_D] \in \mathbb{R}^{N \times D}$ be the visual encoder output, where each column $\mathbf{c}_j \in \mathbb{R}^N$ represents a channel-wise feature vector across $N$ spatial tokens. Our goal is to find an optimal compressed representation $\mathbf{Z}$ that minimizes the IB Lagrangian:
\begin{equation}
    \mathcal{L} = I(\mathbf{X}; \mathbf{Z}) - \beta I(\mathbf{Z}; \mathbf{S}),
\end{equation}
where $\mathbf{S}$ is the target clean code. Following the IB framework for unsupervised clustering, we treat each channel $\mathbf{c}_j$ as a data point (indexed by $j$) to be clustered into $D$ semantic groups (indexed by $c$). We assume the data distribution follows $p(\mathbf{s}|j)=\mathcal{N}(\mathbf{s}|\mathbf{c}_j, \epsilon^2\mathbf{I})$ where $\epsilon$ is a smoothing parameter. The $t$-th iterative step for the soft assignment of channel $j$ to cluster $c$ is given by~\citep{tishby2000information}:
\begin{align}
    \label{eq:ib_iteration}
    q^{(t)}(c|j) &= \frac{p^{(t-1)}(c)}{Z(\mathbf{c}_j, \beta)} \exp\left[ -\beta D_{KL}[p(\mathbf{s}|j) \| p^{(t-1)}(\mathbf{s}|c)] \right],\\
    p^{(t)}(c)&=\frac{n_c^{(t)}}{D},\notag
\end{align}
where $Z(\mathbf{c}_j, \beta)$ is the partition function. We approximate the cluster-conditional distribution $p(\mathbf{s}|c)$ with a Gaussian $g(\mathbf{s}|c) = \mathcal{N}(\mathbf{s}|\boldsymbol{\mu}_c, \Sigma_c)$ and assume $\epsilon$ is sufficiently small. The KL divergence between $p(\mathbf{s}|j)$ and $g(\mathbf{s}|c)$ possesses the closed form:
\begin{align}
    D_{KL}[p(\mathbf{s}|j) \| g(\mathbf{s}|c)] &= \frac{1}{2}\left[ \log\frac{|\Sigma_c|}{|\epsilon^2 \mathbf{I}|} - N + \mathrm{tr}(\Sigma_c^{-1} \epsilon^2 \mathbf{I}) + (\mathbf{c}_j - \boldsymbol{\mu}_c)^\top \Sigma_c^{-1} (\mathbf{c}_j - \boldsymbol{\mu}_c) \right] \notag\\
    &\xrightarrow{\epsilon\to 0} \frac{1}{2}\left[\log |\Sigma_c| + (\mathbf{c}_j - \boldsymbol{\mu}_c)^\top \Sigma_c^{-1} (\mathbf{c}_j - \boldsymbol{\mu}_c)\right] + \mathrm{const} \notag \\
    &\propto (\mathbf{c}_j - \boldsymbol{\mu}_c)^\top \Sigma_c^{-1} (\mathbf{c}_j - \boldsymbol{\mu}_c) + \log |\Sigma_c|. \label{eq:klterm}
\end{align}
Plugging \cref{eq:klterm} into \cref{eq:ib_iteration}, we obtain:
\begin{align}
    q^{(t)}(c|j) =\frac{n_c^{(t-1)}/D}{|\Sigma_c|^{\beta/2}}\frac{\exp\left(-\frac{\beta}{2} (\mathbf{c}_j - \boldsymbol{\mu}_c)^\top \Sigma^{-1} (\mathbf{c}_j - \boldsymbol{\mu}_c) \right)}{Z(\mathbf{c}_j,\beta)}, \notag
\end{align}
where the constant terms are absorbed into the $Z(\mathbf{c}_j,\beta)$. Looking into the quadratic form $(\mathbf{c}_j - \boldsymbol{\mu}_c)^\top \Sigma^{-1} (\mathbf{c}_j - \boldsymbol{\mu}_c)$, for a fixed $j$, the term $\mathbf{c}_j^\top \Sigma^{-1} \mathbf{c}_j$ is constant across all clusters $c$ and can be absorbed into $Z(\mathbf{c}_j, \beta)$. Without loss of generality, we assume a shared covariance $\Sigma_c=\Sigma$ across clusters and normalized cluster centers such that $\boldsymbol{\mu}_c^\top \Sigma^{-1} \boldsymbol{\mu}_c = 1$, we have:
\begin{align}
    q^{(t)}(c|j)=\frac{n_c^{(t-1)}/D}{|\Sigma|^{\beta/2}}\frac{\exp\left(\beta\boldsymbol{\mu}_c^\top \Sigma^{-1}\mathbf{c}_j\right)}{Z(\mathbf{c}_j, \beta)}.\notag
\end{align}
The specific form of the partition function $Z(\mathbf{c}_j, \beta)$ determines the normalization and the resulting attention mechanism. We now consider two cases based on different assumptions about the latent structure.

\paragraph{Case 1: Categorical Latent Structure.} Under the assumption that each channel $j$ must be assigned to \emph{exactly one} cluster, the assignments form a categorical distribution. The partition function enforcing this constraint is $Z(\mathbf{c}_j,\beta) = \sum_{c} \exp\left( \beta \boldsymbol{\mu}_{c}^\top \Sigma^{-1} \mathbf{c}_j \right)$, leading to:
\begin{equation}
   q^{(t)}(c|j)=\frac{n_c^{(t-1)}/D}{|\Sigma|^{\beta/2}}\frac{\exp\left(\beta\boldsymbol{\mu}_c^\top \Sigma^{-1}\mathbf{c}_j\right)}{\sum_{c} \exp\left( \beta \boldsymbol{\mu}_{c}^\top \Sigma^{-1} \mathbf{c}_j \right)}. \notag
\end{equation}
We define the output representation $\mathbf{z}_c^{(t)}$ as these updated cluster centers, i.e.
\begin{align}
    \mathbf{z}_c^{(t)} := \boldsymbol{\mu}_c^{(t)} &=\frac{1}{n_c^{(t)}}\sum_{j=1}^D q^{(t)}(c|j)\mathbf{c}_j=\sum_{j=1}^D \frac{n_c^{(t-1)}/D}{n_c^{(t)}|\Sigma|^{\beta/2}}\frac{\exp\left(\beta\boldsymbol{\mu}_c^\top \Sigma^{-1}\mathbf{c}_j\right)}{\sum_{c} \exp\left( \beta \boldsymbol{\mu}_{c}^\top \Sigma^{-1} \mathbf{c}_j \right)}\\
    &=\sum_{j=1}^D \frac{\exp\left(\beta\mathbf{k}_c^\top \mathbf{q}_j\right)}{\sum_{c} \exp\left(\beta\mathbf{k}_c^\top \mathbf{q}_j\right)}\mathbf{v}_j=\sum_{j=1}^D \text{Softmax}_c(\beta \mathbf{k}_c^\top \mathbf{q}_j)\mathbf{v}_j,
\end{align}
where we define  $\mathbf{q}_j = \Sigma^{-1} \mathbf{c}_j$,  $\mathbf{k}_c = \boldsymbol{\mu}_c^{(t-1)}$ and $\mathbf{v}_j=\frac{n_c^{(t-1)}/D}{n_c^{(t)}|\Sigma|^{\beta/2}}\mathbf{c}_j$. In matrix form, this yields,
\begin{equation}
    \mathbf{Z} = \mathbf{V} \cdot \mathrm{Softmax}\left( \beta \mathbf{Q}^\top \mathbf{K} \right),
\end{equation}
where $\mathbf{Q} = \Sigma^{-1}[\mathbf{c}_1, \dots, \mathbf{c}_D]=\mathbf{W}_Q\mathbf{X}$, $\mathbf{K} = [\boldsymbol{\mu}_1^{(t-1)}, \dots, \boldsymbol{\mu}_D^{(t-1)}]=\mathbf{W}_K\mathbf{X}$ , $\mathbf{V} =\frac{n_c^{(t-1)}/D}{n_c^{(t)}|\Sigma|^{\beta/2}}[\mathbf{c}_1, \dots, \mathbf{c}_D]=\mathbf{W}_V\mathbf{X}$, $\mathbf{Z} = [\boldsymbol{\mu}_1^{(t)}, \dots, \boldsymbol{\mu}_D^{(t)}]$, and $b$ is a learnable bias. Here, $\mathbf{W}_Q,\mathbf{W}_K,\mathbf{W}_V$ are learnable parameters.

\paragraph{Case 2: Independent Bernoulli Latent Structure.} We now relax the categorical constraint. Instead of requiring each channel to be assigned to exactly one semantic group, we assume that the association of channel $j$ with each cluster $c$ is an \emph{independent} binary decision. Let $a_{jc} \in \{0, 1\}$ be a binary latent variable where $a_{jc} = 1$ denotes that channel $j$ is associated with cluster $c$, following an independent Bernoulli distribution. For a specific pair $(j, c)$, the local partition function over the binary state space $\{0, 1\}$ is:
\begin{equation}
    Z(\mathbf{c}_j, \beta) = \exp\left( \beta \boldsymbol{\mu}_c^\top \Sigma^{-1} \mathbf{c}_j \right) + \exp(b),
\end{equation}
where $b$ is a learnable bias representing the activation threshold (the ``off'' state energy). Under this formulation, the probability that channel $j$ carries the semantic information of cluster $c$ is:
\begin{align}
    q^{(t)}(a_{jc}=1 | j) &= \frac{n_c/D}{|\Sigma|^{\beta/2}}\frac{\exp\left( \beta \boldsymbol{\mu}_c^\top \Sigma^{-1} \mathbf{c}_j \right)}{\exp\left( \beta \boldsymbol{\mu}_c^\top \Sigma^{-1} \mathbf{c}_j \right) + \exp(b)}
\end{align}
Similar to the derivation in Case 1, we define the output representation $\mathbf{z}_c^{(t)}$ as these updated cluster centers, i.e.
\begin{align}
    \mathbf{z}_c^{(t)} := \boldsymbol{\mu}_c^{(t)} &= \frac{1}{n_c^{(t)}}\sum_{j=1}^{D} q^{(t)}(a_{jc}=1|j) \cdot \mathbf{c}_j=\sum_{j=1}^{D} \frac{n_c^{(t-1)}/D}{n_c^{(t)}|\Sigma|^{\beta/2}}\frac{\exp\left( \beta \boldsymbol{\mu}_c^\top \Sigma^{-1} \mathbf{c}_j \right)}{\exp\left( \beta \boldsymbol{\mu}_c^\top \Sigma^{-1} \mathbf{c}_j \right) + \exp(b)} \mathbf{c}_j\\
   &= \sum_{j=1}^D \frac{\exp\left(\beta\mathbf{k}_c^\top \mathbf{q}_j\right)}{\exp\left(\beta\mathbf{k}_c^\top \mathbf{q}_j\right)+\exp(b)}\mathbf{v}_j=\sum_{j=1}^D \sigma(\beta\mathbf{k}_c^\top \mathbf{q}_j-b)\mathbf{v}_j,
\end{align}
where we define  $\mathbf{q}_j = \Sigma^{-1} \mathbf{c}_j$,  $\mathbf{k}_c = \boldsymbol{\mu}_c^{(t-1)}$ and $\mathbf{v}_j=\frac{n_c^{(t-1)}/D}{n_c^{(t)}|\Sigma|^{\beta/2}}\mathbf{c}_j$. Here $\sigma(\cdot)=\frac{1}{1+\exp(-x)}$ is the sigmoid activation. In matrix form, this yields,
\begin{equation}
    \mathbf{Z}^{(t)} = \mathbf{V} \cdot \sigma\left( \beta \mathbf{Q}^\top \mathbf{K} - b\mathbf{1}_D\mathbf{1}_D^\top \right).
\end{equation}
where $\mathbf{Q} = \Sigma^{-1}[\mathbf{c}_1, \dots, \mathbf{c}_D]=\mathbf{W}_Q\mathbf{X}$, $\mathbf{K} = [\boldsymbol{\mu}_1^{(t-1)}, \dots, \boldsymbol{\mu}_D^{(t-1)}]=\mathbf{W}_K\mathbf{X}$ , $\mathbf{V} =\frac{n_c^{(t-1)}/D}{n_c^{(t)}|\Sigma|^{\beta/2}}[\mathbf{c}_1, \dots, \mathbf{c}_D]=\mathbf{W}_V\mathbf{X}$, $\mathbf{Z} = [\boldsymbol{\mu}_1^{(t)}, \dots, \boldsymbol{\mu}_D^{(t)}]$, and $b$ is a learnable bias. Here, $\mathbf{W}_Q,\mathbf{W}_K,\mathbf{W}_V$ are learnable parameters. This establishes the functional form of our proposed \nameofmethod.

\paragraph{Remarks.} The core difference lies in the latent competition: the categorical structure forces channels to compete for assignments, enforcing $\sum_c q(c|j) = 1$, whereas the independent Bernoulli structure allows each channel-cluster pair to be evaluated independently. For VLA projectors, {\nameofmethod} is inherently more robust: uncorrelated noise channels exhibit low covariance with all semantic clusters, resulting in gate values near zero ($\sigma \approx 0$), thus effectively filtering nuisances without suppressing legitimate semantic signals.
