# Supplementary material for: Revisiting Chain-of-Thought Reasoning under Limited Supervision: Semi-supervised Chain-of-Thought Learning
Source: arXiv:2607.01511 source file (2026-07-01)
Supplement: Supplementary file 2 [file appendix_b.tex]

\clearpage
\section{Implementation Details}
\label{app:implementation}

\subsection{VLM Pre-training (Alignment Stage)}
\label{app:pretraining}

Since StableVLA introduces the Fused \nameofmethod~projector, a hybrid architecture combining a standard MLP with our covariance-based {\nameofmethod} module, the projector weights differ from standard open-source checkpoints. Therefore, prior to robotic fine-tuning, we perform a Vision-Language Alignment stage to align the visual tokens produced by Fused \nameofmethod~ with the LLM's embedding space.

We strictly adhere to the Prismatic VLMs~\citep{karamcheti2024prismatic} protocol, utilizing the LLaVA-LVIS4V-LRV dataset to ensure general-purpose visual reasoning capabilities. Table~\ref{tab:all_hyperparams} (Top) details the Pre-training configurations.

\subsection{Robotic Fine-tuning \& Baselines}

Following alignment, we fine-tune the model for robotic manipulation. As described in Sec.~\ref{sec:hybrid}, Fused \nameofmethod~ employs a dual-pathway mechanism controlled by a fusion coefficient $\lambda$ and optimized using Stochastic Pathway Dropout ($p_{\text{drop}}$).

To ensure optimal performance, we tailored hyperparameters for different benchmark suites.
Comprehensive hyperparameters for both Pre-training and Fine-tuning across all benchmarks are summarized in Table~\ref{tab:all_hyperparams}.

\textbf{Baseline Configurations.}
To ensure a fair and reproducible comparison, we align all baselines with our evaluation protocol:
\begin{itemize}
    \item \textbf{OpenVLA \citep{kim2024openvla}:} We utilize the official 7B pre-trained checkpoints with standard inference settings.
    \item \textbf{OpenVLA-OFT \citep{kim2025fine-tuning}:} We employ the officially released checkpoints.
    \item \textbf{VLA-Adapter \citep{wang2025vla-adapter}:} For LIBERO, we use official checkpoints.
    For CALVIN, we re-trained the model using the official codebase under identical configurations.
    To ensure a strong baseline, we evaluated checkpoints spanning the convergence trajectory and reported the peak performance.\footnote{Specifically, we evaluated checkpoints at different training stages, yielding scores of 3.601, 4.14, 3.628, 3.92, and 4.097. We report the best result (4.14) to represent the baseline's upper bound capability.}
    \item \textbf{OpenPi ($\pi_{0.5}$) \citep{DBLP:journals/corr/abs-2504-16054}:} We utilize the officially released model weights and follow the standard evaluation protocol provided by the authors.
\end{itemize}

\begin{table}[h!]
    \centering
    \caption{Detailed Hyperparameters for StableVLA across Pre-training and Fine-tuning stages.}
    \label{tab:all_hyperparams}
    \begin{tabular}{l|cccc|c}
        \toprule
        \multicolumn{6}{c}{\textbf{Stage I: Vision-Language Pre-training}} \\
        \midrule
        \multicolumn{1}{l|}{\textbf{Base Components}} & \multicolumn{5}{l}{LLM: Qwen2.5-0.5B \quad Vision: DINO-SigLIP (224px)} \\
        \multicolumn{1}{l|}{\textbf{Optimization}} & \multicolumn{5}{l}{Global Batch: 64 \quad LR: 2e-5 \quad Precision: BF16} \\
        \multicolumn{1}{l|}{\textbf{Fused \nameofmethod~ Params}} & \multicolumn{5}{l}{Fusion Coeff. ($\lambda$): 0.3 \quad Pathway Dropout ($p_{\text{drop}}$): 0.0} \\
        \midrule
        \midrule
        \multicolumn{6}{c}{\textbf{Stage II: Robotic Fine-tuning}} \\
        \midrule
        & \multicolumn{4}{c|}{\textbf{LIBERO Benchmark}} & \textbf{CALVIN} \\
        \cmidrule(lr){2-5} \cmidrule(lr){6-6}
        \textbf{Hyperparameter} & \textbf{Spatial} & \textbf{Goal} & \textbf{Long} & \textbf{Object} & \textbf{Benchmark} \\
        \midrule
        Global Batch Size & 64 & 128 & 128 & 64 & 64 \\
        Learning Rate & 2e-4 & 2e-4 & 2e-4 & 2e-4 & 2e-4 \\
        LoRA Rank & 64 & 64 & 64 & 64 & 64 \\
        \midrule
        \multicolumn{6}{l}{\textit{Fused \nameofmethod~ Specific Parameters (Ours)}} \\
        Fusion Coeff. ($\lambda$) & 0.3 & 0.3 & 0.3 & 0.3 & 0.3 \\
        Pathway Dropout ($p_{\text{drop}}$) & 0.3 & 0.4 & 0.0 & 0.3 & 0.3 \\
        \bottomrule
    \end{tabular}
\end{table}
