# Supplementary material for: Revisiting Chain-of-Thought Reasoning under Limited Supervision: Semi-supervised Chain-of-Thought Learning
Source: arXiv:2607.01511 source file (2026-07-01)
Supplement: Supplementary file 3 [file appendix_c.tex]

\clearpage
\section{Detailed Experimental Results}
  \label{app:detailed_results}

  In this appendix, we provide comprehensive quantitative results for all methods evaluated in our experiments.

  \subsection{Full Comparison on LIBERO}

  Table~\ref{tab:app_full_libero} presents the complete comparison of all methods on the LIBERO benchmark, grouped by their training paradigm. Methods are categorized into three groups: (1) \textit{OpenX Pretrain}, which includes models pretrained on the Open X-Embodiment dataset; (2) \textit{OpenX + Web Co-train}, which additionally incorporates web data during pretraining; and (3) \textit{VLM Direct FT}, which directly fine-tunes from vision-language models without robot-specific pretraining.

  % Appendix Table: Full comparison on LIBERO benchmark (grouped by training paradigm)
% Auto-generated from CSV data
\begin{table}[h]
\centering
\setlength{\tabcolsep}{3.5pt}
\footnotesize
\caption{Full comparison on LIBERO benchmark. Methods are grouped by training paradigm. We report success rate (\%). \textbf{Bold}: best, \underline{underline}: second best.}
\label{tab:app_full_libero}
\begin{tabular}{p{1.2cm}l cccc cccc cccc cccc}
\toprule
 & & \multicolumn{4}{c}{Spatial} & \multicolumn{4}{c}{Object} & \multicolumn{4}{c}{Goal} & \multicolumn{4}{c}{Long} \\
\cmidrule(lr){3-6} \cmidrule(lr){7-10} \cmidrule(lr){11-14} \cmidrule(lr){15-18}
Training & Method & C & S3 & S4 & S5 & C & S3 & S4 & S5 & C & S3 & S4 & S5 & C & S3 & S4 & S5 \\
\midrule
\multirow{2}{1.2cm}{\raggedright\scriptsize OpenX\\Pretrain} & OpenVLA & 80.0 & 40.9 & 24.6 & 14.7 & 69.6 & 18.2 & 10.4 & 2.7 & 74.0 & 38.7 & 27.0 & 16.3 & 55.5 & 20.5 & 12.4 & 7.0 \\
 & OpenVLA-OFT & 92.6 & 89.3 & \underline{84.0} & \underline{72.1} & 98.4 & 82.5 & 69.2 & 52.8 & 96.8 & \textbf{94.5} & \underline{84.6} & \underline{70.3} & \textbf{94.4} & \textbf{77.6} & 61.9 & 40.3 \\
\midrule
\multirow{1}{1.2cm}[8pt]{\raggedright\scriptsize OpenX +\\Web Co-train} & 
\rule[-10pt]{0pt}{24pt} OpenPI0.5 & \textbf{98.4} & 88.3 & 79.0 & 62.4 & \textbf{99.4} & \textbf{97.1} & \textbf{88.4} & \textbf{76.4} & 97.2 & 87.2 & 82.5 & 64.2 & 92.0 & 76.1 & \textbf{65.6} & \textbf{47.7} \\
\midrule
\multirow{2}{1.2cm}{\raggedright\scriptsize VLM\\Direct FT} & VLA-Adapter-Pro & 96.0 & \underline{93.7} & 83.3 & 58.5 & 96.8 & 71.0 & 44.1 & 29.3 & \underline{97.4} & 79.5 & 64.7 & 47.3 & \underline{94.4} & 63.5 & 41.0 & 26.2 \\
 & StableVLA & \underline{96.2} & \textbf{94.3} & \textbf{92.1} & \textbf{82.0} & \underline{98.8} & \underline{92.4} & \underline{83.6} & \underline{70.2} & \textbf{98.0} & \underline{93.4} & \textbf{85.0} & \textbf{71.9} & 93.6 & \underline{76.3} & \underline{62.4} & \underline{45.3} \\
\bottomrule
\end{tabular}
\end{table}

  \subsection{Per-Method Detailed Results}

  The following tables provide detailed per-corruption-type results for each method. Each table reports performance across all 19 corruption types (18 for tasks without Glass Blur) at severity levels 3, 4, and 5, along with clean (uncorrupted) performance.

  \paragraph{StableVLA (Ours).} Table~\ref{tab:detail_stablevla} shows the detailed results for our method on both LIBERO and CALVIN benchmarks.

  % Detailed results for StableVLA
% Auto-generated from CSV data
\begin{table}[h]
\centering
\setlength{\tabcolsep}{5pt}
\caption{Detailed results for StableVLA on LIBERO and CALVIN benchmarks. We report success rate (\%) for LIBERO and average completed tasks for CALVIN.}
\label{tab:detail_stablevla}
\begin{tabular}{l ccc ccc ccc ccc ccc}
\toprule
 & \multicolumn{12}{c}{LIBERO} & \multicolumn{3}{c}{CALVIN} \\
\cmidrule(lr){2-13} \cmidrule(lr){14-16}
 & \multicolumn{3}{c}{Spatial} & \multicolumn{3}{c}{Object} & \multicolumn{3}{c}{Goal} & \multicolumn{3}{c}{Long} & \multicolumn{3}{c}{-} \\
\cmidrule(lr){2-4} \cmidrule(lr){5-7} \cmidrule(lr){8-10} \cmidrule(lr){11-13} \cmidrule(lr){14-16}
Corruption & S3 & S4 & S5 & S3 & S4 & S5 & S3 & S4 & S5 & S3 & S4 & S5 & S3 & S4 & S5 \\
\midrule
Clean & 96.2 & - & - & 98.8 & - & - & 98.0 & - & - & 93.6 & - & - & 4.17 & - & - \\
Gaussian Noise & 96.0 & 92.8 & 74.0 & 95.4 & 85.0 & 64.8 & 95.2 & 85.2 & 53.2 & 82.8 & 53.6 & 25.0 & 2.02 & 1.26 & 0.60 \\
Shot Noise & 95.4 & 88.0 & 71.0 & 93.2 & 80.6 & 64.0 & 96.2 & 81.4 & 61.8 & 84.8 & 63.0 & 23.4 & 1.85 & 0.82 & 0.46 \\
Impulse Noise & 94.6 & 93.2 & 80.8 & 96.0 & 83.2 & 62.8 & 96.2 & 81.8 & 57.2 & 81.2 & 55.2 & 30.2 & 2.60 & 1.32 & 0.72 \\
Speckle Noise & 94.6 & 96.6 & 90.4 & 95.6 & 93.2 & 87.2 & 97.8 & 96.0 & 86.4 & 87.2 & 84.0 & 71.8 & 2.16 & 1.49 & 0.90 \\
Gaussian Blur & 91.6 & 83.0 & 49.4 & 84.4 & 45.4 & 2.4 & 91.8 & 74.0 & 42.6 & 55.4 & 31.2 & 2.8 & 2.18 & 0.94 & 0.34 \\
Glass Blur & 91.2 & 83.6 & 55.8 & - & - & - & - & - & - & - & - & - & - & - & - \\
Defocus Blur & 89.4 & 81.6 & 65.0 & 72.8 & 46.8 & 24.8 & 85.8 & 63.0 & 47.2 & 49.6 & 27.2 & 10.6 & 1.56 & 0.64 & 0.34 \\
Motion Blur & 89.6 & 90.4 & 82.6 & 98.2 & 72.0 & 27.4 & 93.4 & 59.8 & 37.6 & 66.0 & 21.6 & 1.0 & 1.23 & 0.46 & 0.24 \\
Zoom Blur & 95.8 & 93.6 & 86.2 & 60.8 & 49.8 & 46.8 & 91.0 & 82.8 & 69.0 & 36.8 & 16.8 & 11.2 & 3.48 & 2.86 & 2.10 \\
Fog & 95.0 & 94.0 & 94.4 & 99.8 & 99.6 & 94.8 & 94.4 & 95.2 & 81.4 & 78.4 & 75.0 & 57.0 & 2.84 & 1.97 & 0.88 \\
Frost & 96.0 & 93.8 & 89.8 & 84.0 & 79.4 & 67.4 & 92.0 & 88.6 & 81.0 & 72.6 & 69.2 & 54.8 & 3.11 & 2.99 & 2.64 \\
Snow & 95.4 & 94.8 & 94.2 & 97.4 & 92.2 & 95.4 & 92.0 & 85.4 & 95.4 & 61.0 & 39.2 & 33.0 & 3.45 & 2.50 & 1.62 \\
Spatter & 96.6 & 95.0 & 95.2 & 98.2 & 98.6 & 93.4 & 93.8 & 94.4 & 91.2 & 90.8 & 94.4 & 87.2 & 4.13 & 4.04 & 3.74 \\
Contrast & 94.2 & 95.2 & 68.0 & 99.0 & 98.4 & 78.6 & 97.6 & 95.6 & 56.8 & 93.6 & 90.2 & 52.6 & 3.74 & 2.30 & 0.59 \\
Brightness & 96.4 & 96.2 & 97.0 & 98.4 & 99.0 & 98.4 & 98.0 & 99.0 & 98.0 & 92.4 & 90.2 & 90.6 & 4.04 & 3.48 & 2.71 \\
Saturate & 96.6 & 96.4 & 98.0 & 98.8 & 98.2 & 97.2 & 96.6 & 98.2 & 97.8 & 93.4 & 92.0 & 89.8 & 4.20 & 4.19 & 4.17 \\
JPEG Comp. & 96.2 & 96.6 & 94.4 & 98.6 & 98.8 & 97.4 & 96.8 & 97.4 & 96.8 & 89.4 & 88.8 & 73.8 & 2.79 & 2.42 & 1.50 \\
Pixelate & 94.6 & 95.2 & 94.4 & 96.4 & 96.4 & 95.6 & 97.6 & 96.8 & 95.6 & 92.8 & 93.0 & 84.6 & 2.60 & 2.86 & 2.69 \\
Elastic Trans. & 91.6 & 90.4 & 78.2 & 95.6 & 89.0 & 65.8 & 74.4 & 55.2 & 45.2 & 65.2 & 38.8 & 16.2 & 1.94 & 1.49 & 0.99 \\
\bottomrule
\end{tabular}
\end{table}

  \paragraph{VLA-Adapter-Pro.} Table~\ref{tab:detail_vla_adapter_pro} presents results for VLA-Adapter-Pro, the strongest baseline that shares our VLM direct fine-tuning paradigm.

  % Detailed results for VLA-Adapter-Pro
% Auto-generated from CSV data
\begin{table}[h]
\centering
\setlength{\tabcolsep}{5pt}
\caption{Detailed results for VLA-Adapter-Pro on LIBERO and CALVIN benchmarks. We report success rate (\%) for LIBERO and average completed tasks for CALVIN.}
\label{tab:detail_vla_adapter_pro}
\begin{tabular}{l ccc ccc ccc ccc ccc}
\toprule
 & \multicolumn{12}{c}{LIBERO} & \multicolumn{3}{c}{CALVIN} \\
\cmidrule(lr){2-13} \cmidrule(lr){14-16}
 & \multicolumn{3}{c}{Spatial} & \multicolumn{3}{c}{Object} & \multicolumn{3}{c}{Goal} & \multicolumn{3}{c}{Long} & \multicolumn{3}{c}{-} \\
\cmidrule(lr){2-4} \cmidrule(lr){5-7} \cmidrule(lr){8-10} \cmidrule(lr){11-13} \cmidrule(lr){14-16}
Corruption & S3 & S4 & S5 & S3 & S4 & S5 & S3 & S4 & S5 & S3 & S4 & S5 & S3 & S4 & S5 \\
\midrule
Clean & 96.0 & - & - & 96.8 & - & - & 97.4 & - & - & 94.4 & - & - & 4.14 & - & - \\
Gaussian Noise & 98.2 & 93.8 & 32.4 & 97.2 & 53.8 & 0.0 & 79.4 & 53.4 & 26.0 & 69.4 & 37.0 & 1.0 & 2.35 & 1.03 & 0.29 \\
Shot Noise & 97.8 & 84.6 & 12.8 & 93.8 & 23.4 & 0.0 & 74.6 & 49.2 & 36.6 & 76.4 & 22.8 & 4.0 & 2.06 & 0.80 & 0.21 \\
Impulse Noise & 99.0 & 93.2 & 38.0 & 98.8 & 67.8 & 0.0 & 77.4 & 56.8 & 26.4 & 72.0 & 38.6 & 2.6 & 2.92 & 1.14 & 0.37 \\
Speckle Noise & 97.8 & 97.4 & 85.0 & 97.2 & 85.4 & 40.0 & 75.2 & 67.8 & 54.6 & 83.2 & 71.2 & 28.2 & 2.59 & 1.76 & 0.90 \\
Gaussian Blur & 89.2 & 56.2 & 3.8 & 28.0 & 0.0 & 0.0 & 87.6 & 72.6 & 26.8 & 37.0 & 3.2 & 0.0 & 0.76 & 0.12 & 0.00 \\
Glass Blur & 72.6 & 41.4 & 8.0 & - & - & - & - & - & - & - & - & - & - & - & - \\
Defocus Blur & 77.8 & 35.6 & 6.6 & 5.0 & 0.0 & 0.0 & 81.6 & 60.0 & 36.4 & 19.6 & 1.4 & 0.0 & 0.41 & 0.06 & 0.00 \\
Motion Blur & 88.0 & 59.2 & 29.0 & 11.6 & 0.0 & 0.0 & 89.2 & 47.2 & 21.4 & 36.2 & 8.0 & 0.0 & 0.69 & 0.08 & 0.01 \\
Zoom Blur & 87.8 & 78.0 & 71.8 & 19.2 & 6.0 & 0.0 & 73.2 & 59.0 & 41.0 & 9.0 & 1.2 & 2.0 & 2.95 & 2.43 & 1.76 \\
Fog & 98.6 & 98.0 & 93.6 & 63.4 & 11.8 & 0.2 & 77.4 & 71.0 & 46.2 & 52.4 & 37.0 & 12.6 & 2.77 & 2.38 & 1.34 \\
Frost & 93.8 & 90.2 & 81.4 & 32.2 & 22.8 & 8.2 & 59.8 & 55.0 & 43.2 & 49.4 & 36.4 & 19.0 & 3.61 & 3.46 & 3.37 \\
Snow & 97.2 & 91.6 & 95.6 & 63.0 & 7.6 & 59.2 & 58.2 & 40.6 & 57.0 & 41.8 & 6.0 & 13.6 & 3.64 & 3.03 & 2.73 \\
Spatter & 98.4 & 96.6 & 88.0 & 97.2 & 53.4 & 6.0 & 89.2 & 77.6 & 61.0 & 82.4 & 68.2 & 36.2 & 4.05 & 3.93 & 3.23 \\
Contrast & 99.4 & 97.8 & 25.8 & 88.6 & 0.0 & 0.0 & 91.4 & 79.0 & 26.0 & 68.6 & 4.4 & 0.0 & 2.54 & 0.78 & 0.01 \\
Brightness & 98.2 & 99.4 & 97.8 & 98.8 & 98.4 & 98.6 & 89.8 & 89.6 & 88.2 & 91.2 & 91.4 & 86.0 & 4.16 & 4.12 & 3.74 \\
Saturate & 99.2 & 99.2 & 99.2 & 98.4 & 98.4 & 94.0 & 98.0 & 92.8 & 88.0 & 93.8 & 80.8 & 84.0 & 4.13 & 4.13 & 4.14 \\
JPEG Comp. & 99.0 & 98.2 & 98.6 & 98.4 & 98.8 & 98.8 & 87.4 & 84.4 & 81.6 & 90.4 & 88.8 & 81.4 & 1.80 & 1.14 & 0.53 \\
Pixelate & 98.2 & 97.2 & 94.8 & 96.2 & 91.0 & 80.0 & 97.0 & 95.0 & 88.6 & 89.6 & 85.0 & 69.4 & 2.65 & 2.01 & 1.94 \\
Elastic Trans. & 90.2 & 74.8 & 50.2 & 90.8 & 75.0 & 42.6 & 44.2 & 14.2 & 2.8 & 80.4 & 56.8 & 31.8 & 1.89 & 1.61 & 1.26 \\
\bottomrule
\end{tabular}
\end{table}

  \paragraph{OpenVLA.} Table~\ref{tab:detail_openvla} shows results for the base OpenVLA model.

  % Detailed results for OpenVLA
% Auto-generated from CSV data
\begin{table}[t]
\centering
\setlength{\tabcolsep}{6pt}
\caption{Detailed results for OpenVLA on LIBERO benchmark. We report success rate (\%).}
\label{tab:detail_openvla}
\begin{tabular}{l ccc ccc ccc ccc}
\toprule
 & \multicolumn{3}{c}{Spatial} & \multicolumn{3}{c}{Object} & \multicolumn{3}{c}{Goal} & \multicolumn{3}{c}{Long} \\
\cmidrule(lr){2-4} \cmidrule(lr){5-7} \cmidrule(lr){8-10} \cmidrule(lr){11-13}
Corruption & S3 & S4 & S5 & S3 & S4 & S5 & S3 & S4 & S5 & S3 & S4 & S5 \\
\midrule
Clean & 80.0 & - & - & 69.6 & - & - & 74.0 & - & - & 55.5 & - & - \\
Gaussian Noise & 50.2 & 0.6 & 0.0 & 0.6 & 0.0 & 0.0 & 31.4 & 4.8 & 0.0 & 8.4 & 0.2 & 0.0 \\
Shot Noise & 39.0 & 0.0 & 0.0 & 0.4 & 0.0 & 0.0 & 23.6 & 2.8 & 0.0 & 5.6 & 0.0 & 0.0 \\
Impulse Noise & 55.2 & 1.4 & 0.0 & 3.0 & 0.0 & 0.0 & 41.0 & 4.8 & 0.0 & 9.2 & 1.6 & 0.0 \\
Speckle Noise & 61.0 & 26.0 & 2.8 & 5.2 & 0.2 & 0.0 & 40.8 & 17.2 & 8.4 & 17.6 & 3.8 & 0.0 \\
Gaussian Blur & 0.0 & 0.0 & 0.0 & 0.0 & 0.0 & 0.0 & 2.4 & 0.2 & 0.0 & 0.0 & 0.0 & 0.0 \\
Glass Blur & 0.0 & 0.0 & 0.0 & - & - & - & - & - & - & - & - & - \\
Defocus Blur & 0.0 & 0.0 & 0.0 & 0.0 & 0.0 & 0.0 & 0.4 & 0.2 & 0.8 & 0.0 & 0.0 & 0.0 \\
Motion Blur & 0.0 & 0.0 & 0.0 & 0.0 & 0.0 & 0.0 & 0.6 & 0.0 & 0.0 & 0.0 & 0.0 & 0.0 \\
Zoom Blur & 7.6 & 3.2 & 0.2 & 0.6 & 0.0 & 0.0 & 14.0 & 3.4 & 1.6 & 3.0 & 0.2 & 0.0 \\
Fog & 74.6 & 69.4 & 38.0 & 46.4 & 24.2 & 0.4 & 76.2 & 69.0 & 40.2 & 51.0 & 46.4 & 20.2 \\
Frost & 20.2 & 16.8 & 4.4 & 0.6 & 0.2 & 0.4 & 28.4 & 22.8 & 14.0 & 15.6 & 12.0 & 4.2 \\
Snow & 39.0 & 10.4 & 22.2 & 0.4 & 0.0 & 0.0 & 28.6 & 19.8 & 15.0 & 14.6 & 2.2 & 3.2 \\
Spatter & 65.4 & 32.4 & 3.8 & 14.2 & 0.2 & 0.0 & 50.2 & 37.0 & 16.2 & 36.0 & 12.6 & 2.2 \\
Contrast & 71.2 & 52.6 & 6.8 & 57.4 & 28.0 & 0.0 & 75.0 & 69.2 & 16.8 & 50.2 & 38.8 & 10.0 \\
Brightness & 78.4 & 73.8 & 62.8 & 64.6 & 53.2 & 29.0 & 76.0 & 73.4 & 60.8 & 52.6 & 45.6 & 41.2 \\
Saturate & 80.8 & 81.4 & 74.2 & 65.8 & 47.8 & 12.6 & 75.2 & 75.2 & 69.8 & 55.6 & 48.6 & 40.2 \\
JPEG Comp. & 72.4 & 69.8 & 56.6 & 42.6 & 29.4 & 5.8 & 73.8 & 63.2 & 45.0 & 31.8 & 10.0 & 4.2 \\
Pixelate & 60.0 & 29.0 & 7.2 & 24.8 & 3.6 & 0.0 & 53.6 & 21.2 & 5.2 & 15.4 & 1.0 & 0.0 \\
Elastic Trans. & 2.6 & 0.2 & 0.0 & 1.0 & 0.2 & 0.0 & 5.4 & 1.8 & 0.4 & 3.2 & 1.0 & 0.0 \\
\bottomrule
\end{tabular}
\end{table}

  \paragraph{OpenVLA-OFT.} Table~\ref{tab:detail_openvla_oft} presents results for OpenVLA with orthogonal fine-tuning.

  % Detailed results for OpenVLA-OFT
% Auto-generated from CSV data
\begin{table}[t]
\centering
\setlength{\tabcolsep}{6pt}
\caption{Detailed results for OpenVLA-OFT on LIBERO benchmark. We report success rate (\%).}
\label{tab:detail_openvla_oft}
\begin{tabular}{l ccc ccc ccc ccc}
\toprule
 & \multicolumn{3}{c}{Spatial} & \multicolumn{3}{c}{Object} & \multicolumn{3}{c}{Goal} & \multicolumn{3}{c}{Long} \\
\cmidrule(lr){2-4} \cmidrule(lr){5-7} \cmidrule(lr){8-10} \cmidrule(lr){11-13}
Corruption & S3 & S4 & S5 & S3 & S4 & S5 & S3 & S4 & S5 & S3 & S4 & S5 \\
\midrule
Clean & 92.6 & - & - & 98.4 & - & - & 96.8 & - & - & 94.4 & - & - \\
Gaussian Noise & 90.4 & 89.2 & 67.8 & 88.6 & 56.4 & 21.2 & 94.4 & 87.2 & 56.0 & 74.6 & 47.6 & 13.8 \\
Shot Noise & 90.8 & 85.4 & 70.2 & 88.0 & 85.4 & 70.2 & 97.0 & 76.0 & 57.4 & 82.4 & 45.6 & 12.0 \\
Impulse Noise & 90.2 & 85.6 & 64.8 & 90.2 & 56.0 & 25.8 & 95.6 & 84.0 & 56.4 & 80.2 & 48.0 & 18.8 \\
Speckle Noise & 92.4 & 90.0 & 84.4 & 91.4 & 83.6 & 56.8 & 96.6 & 94.2 & 80.8 & 88.4 & 81.0 & 47.0 \\
Gaussian Blur & 86.8 & 80.6 & 46.6 & 53.0 & 35.0 & 4.6 & 96.4 & 84.8 & 48.0 & 78.0 & 38.4 & 6.2 \\
Glass Blur & 84.4 & 73.6 & 42.6 & - & - & - & - & - & - & - & - & - \\
Defocus Blur & 85.6 & 69.4 & 46.8 & 47.6 & 27.6 & 11.2 & 93.0 & 76.8 & 53.4 & 57.8 & 30.2 & 11.0 \\
Motion Blur & 77.6 & 55.6 & 39.4 & 57.4 & 20.6 & 3.8 & 89.6 & 51.6 & 27.8 & 42.6 & 16.0 & 4.6 \\
Zoom Blur & 82.2 & 71.8 & 62.6 & 70.8 & 44.0 & 30.8 & 87.4 & 77.6 & 69.6 & 54.8 & 38.2 & 13.4 \\
Fog & 90.4 & 87.8 & 73.0 & 94.0 & 85.6 & 59.2 & 96.0 & 92.0 & 63.0 & 81.6 & 71.0 & 37.8 \\
Frost & 91.6 & 89.0 & 83.0 & 84.0 & 80.8 & 83.0 & 90.6 & 83.8 & 70.2 & 69.2 & 61.4 & 54.2 \\
Snow & 92.4 & 89.2 & 93.0 & 88.2 & 80.2 & 61.4 & 89.6 & 64.6 & 83.0 & 61.6 & 35.2 & 29.0 \\
Spatter & 93.2 & 90.0 & 84.0 & 96.6 & 92.6 & 86.4 & 95.4 & 90.8 & 84.6 & 88.6 & 90.8 & 71.8 \\
Contrast & 91.8 & 89.4 & 69.6 & 96.0 & 90.6 & 56.8 & 98.4 & 93.2 & 66.2 & 91.0 & 84.6 & 32.4 \\
Brightness & 93.8 & 94.2 & 92.4 & 96.0 & 94.8 & 93.0 & 99.0 & 98.2 & 97.6 & 91.2 & 91.8 & 90.0 \\
Saturate & 92.8 & 92.4 & 92.8 & 92.8 & 95.4 & 94.0 & 95.4 & 95.0 & 97.6 & 91.6 & 91.8 & 85.2 \\
JPEG Comp. & 92.2 & 92.2 & 92.6 & 97.0 & 96.8 & 91.8 & 98.6 & 96.0 & 97.2 & 92.0 & 87.4 & 83.8 \\
Pixelate & 91.6 & 90.8 & 90.4 & 86.2 & 69.6 & 64.2 & 97.0 & 97.4 & 96.6 & 91.8 & 90.0 & 84.6 \\
Elastic Trans. & 86.6 & 80.2 & 74.4 & 66.6 & 51.2 & 36.0 & 90.6 & 79.8 & 60.2 & 80.0 & 65.2 & 29.6 \\
\bottomrule
\end{tabular}
\end{table}

  \paragraph{OpenPI.} Table~\ref{tab:detail_openpi} shows results for OpenPI, which leverages internet-scale co-training.

  % Detailed results for OpenPI
% Auto-generated from CSV data
\begin{table}[t]
\centering
\setlength{\tabcolsep}{6pt}
\caption{Detailed results for OpenPI on LIBERO benchmark. We report success rate (\%).}
\label{tab:detail_openpi}
\begin{tabular}{l ccc ccc ccc ccc}
\toprule
 & \multicolumn{3}{c}{Spatial} & \multicolumn{3}{c}{Object} & \multicolumn{3}{c}{Goal} & \multicolumn{3}{c}{Long} \\
\cmidrule(lr){2-4} \cmidrule(lr){5-7} \cmidrule(lr){8-10} \cmidrule(lr){11-13}
Corruption & S3 & S4 & S5 & S3 & S4 & S5 & S3 & S4 & S5 & S3 & S4 & S5 \\
\midrule
Clean & 98.4 & - & - & 99.4 & - & - & 97.2 & - & - & 92.0 & - & - \\
Gaussian Noise & 98.4 & 92.0 & 29.8 & 98.4 & 98.0 & 58.4 & 96.2 & 78.0 & 21.6 & 88.4 & 73.2 & 13.0 \\
Shot Noise & 98.0 & 75.0 & 24.2 & 98.8 & 95.8 & 53.0 & 94.0 & 79.6 & 31.8 & 89.4 & 72.6 & 29.8 \\
Impulse Noise & 98.4 & 94.8 & 36.0 & 99.4 & 98.6 & 62.0 & 95.2 & 79.4 & 28.2 & 90.0 & 73.4 & 17.6 \\
Speckle Noise & 97.6 & 98.0 & 77.8 & 98.4 & 98.6 & 96.6 & 96.6 & 92.6 & 86.6 & 87.0 & 83.6 & 79.0 \\
Gaussian Blur & 41.4 & 10.8 & 0.0 & 88.8 & 10.0 & 0.0 & 76.4 & 44.6 & 1.6 & 11.0 & 0.4 & 0.0 \\
Glass Blur & 59.8 & 39.2 & 9.0 & - & - & - & - & - & - & - & - & - \\
Defocus Blur & 43.2 & 17.6 & 6.8 & 83.0 & 32.4 & 0.8 & 69.2 & 47.2 & 11.6 & 10.6 & 0.6 & 0.0 \\
Motion Blur & 81.6 & 38.4 & 10.8 & 96.2 & 77.8 & 34.8 & 87.0 & 55.0 & 24.4 & 62.4 & 21.6 & 1.2 \\
Zoom Blur & 80.4 & 75.8 & 74.4 & 99.4 & 98.4 & 97.4 & 89.6 & 83.2 & 77.0 & 60.0 & 0.8 & 1.0 \\
Fog & 96.8 & 92.0 & 81.0 & 98.4 & 99.0 & 97.2 & 97.0 & 96.0 & 82.4 & 87.6 & 76.4 & 50.2 \\
Frost & 95.8 & 91.0 & 77.4 & 98.8 & 98.8 & 95.4 & 85.8 & 81.6 & 72.4 & 47.6 & 74.2 & 56.2 \\
Snow & 97.2 & 91.8 & 91.4 & 99.4 & 98.2 & 98.2 & 92.8 & 77.8 & 79.8 & 89.6 & 76.0 & 40.8 \\
Spatter & 99.0 & 98.0 & 96.0 & 98.6 & 99.6 & 99.4 & 96.8 & 96.8 & 93.0 & 94.0 & 93.6 & 90.0 \\
Contrast & 98.4 & 97.0 & 94.0 & 98.6 & 99.0 & 96.0 & 98.0 & 97.2 & 93.6 & 89.6 & 88.6 & 67.4 \\
Brightness & 98.2 & 98.2 & 98.0 & 98.8 & 99.2 & 99.4 & 8.2 & 97.2 & 97.0 & 92.2 & 91.8 & 93.2 \\
Saturate & 99.2 & 99.0 & 98.4 & 97.6 & 98.2 & 98.8 & 98.4 & 97.0 & 97.2 & 92.8 & 92.2 & 94.0 \\
JPEG Comp. & 96.0 & 97.2 & 96.8 & 98.4 & 99.2 & 99.0 & 96.2 & 95.0 & 95.8 & 88.6 & 88.2 & 88.2 \\
Pixelate & 99.4 & 96.8 & 88.2 & 98.0 & 90.4 & 88.0 & 97.4 & 96.4 & 80.6 & 93.6 & 83.4 & 55.8 \\
Elastic Trans. & 99.2 & 97.8 & 96.0 & 99.6 & 99.8 & 100.0 & 94.8 & 90.4 & 81.4 & 95.0 & 90.0 & 81.6 \\
\bottomrule
\end{tabular}
\end{table}

  \subsection{Ablation Study Details}

  The following tables provide detailed results for our ablation study on adapter architecture design.

  \paragraph{IB-Adapter.} Table~\ref{tab:detail_ib_adapter} shows results for IB-Adapter, which uses only the image-bridge component without feature fusion.

  % Detailed results for IB-Adapter
% Auto-generated from CSV data
\begin{table}[t]
\centering
\setlength{\tabcolsep}{5pt}
\caption{Detailed results for IB-Adapter on LIBERO and CALVIN benchmarks. We report success rate (\%) for LIBERO and average completed tasks for CALVIN.}
\label{tab:detail_ib_adapter}
\begin{tabular}{l ccc ccc ccc ccc ccc}
\toprule
 & \multicolumn{12}{c}{LIBERO} & \multicolumn{3}{c}{CALVIN} \\
\cmidrule(lr){2-13} \cmidrule(lr){14-16}
 & \multicolumn{3}{c}{Spatial} & \multicolumn{3}{c}{Object} & \multicolumn{3}{c}{Goal} & \multicolumn{3}{c}{Long} & \multicolumn{3}{c}{-} \\
\cmidrule(lr){2-4} \cmidrule(lr){5-7} \cmidrule(lr){8-10} \cmidrule(lr){11-13} \cmidrule(lr){14-16}
Corruption & S3 & S4 & S5 & S3 & S4 & S5 & S3 & S4 & S5 & S3 & S4 & S5 & S3 & S4 & S5 \\
\midrule
Clean & 97.8 & - & - & 0.97 & - & - & 97.4 & - & - & 93.8 & - & - & 1.64 & - & - \\
Gaussian Noise & 95.2 & 94.2 & 79.4 & 96.6 & 80.0 & 15.0 & 85.8 & 78.0 & 57.2 & 88.0 & 54.4 & 9.8 & 1.61 & 1.58 & 1.47 \\
Shot Noise & 96.0 & 91.4 & 76.6 & 95.4 & 67.8 & 15.0 & 86.4 & 70.6 & 62.6 & 84.8 & 56.2 & 1.7 & 1.63 & 1.61 & 1.43 \\
Impulse Noise & 97.4 & 95.0 & 84.0 & 97.4 & 86.2 & 23.4 & 89.0 & 77.0 & 55.4 & 87.0 & 54.8 & 12.4 & 1.66 & 1.60 & 1.50 \\
Speckle Noise & 96.8 & 96.2 & 91.4 & 96.6 & 97.0 & 92.2 & 84.2 & 84.2 & 77.2 & 89.4 & 80.0 & 58.4 & 1.55 & 1.54 & 1.37 \\
Gaussian Blur & 88.6 & 80.8 & 32.4 & 88.0 & 36.6 & 2.0 & 93.6 & 86.0 & 68.4 & 56.0 & 41.2 & 5.2 & 1.52 & 1.44 & 1.26 \\
Glass Blur & 89.4 & 75.4 & 43.2 & - & - & - & - & - & - & - & - & - & - & - & - \\
Defocus Blur & 88.0 & 78.6 & 45.4 & 85.2 & 35.6 & 17.4 & 89.2 & 79.6 & 68.4 & 50.6 & 37.4 & 13.6 & 1.53 & 1.46 & 1.32 \\
Motion Blur & 93.0 & 87.6 & 74.6 & 91.4 & 40.6 & 2.0 & 91.2 & 75.2 & 56.0 & 71.0 & 21.0 & 1.8 & 1.44 & 1.23 & 1.16 \\
Zoom Blur & 96.0 & 90.4 & 88.0 & 50.4 & 13.2 & 12.0 & 92.6 & 83.4 & 66.6 & 44.0 & 18.5 & 10.4 & 1.54 & 1.59 & 1.48 \\
Fog & 98.4 & 98.0 & 93.4 & 96.4 & 96.4 & 56.8 & 86.6 & 86.0 & 65.4 & 87.6 & 81.4 & 52.2 & 1.11 & 1.09 & 0.92 \\
Frost & 95.2 & 93.8 & 89.4 & 94.0 & 85.8 & 69.8 & 75.0 & 70.4 & 63.0 & 68.8 & 60.8 & 43.2 & 1.70 & 1.66 & 1.61 \\
Snow & 98.8 & 97.4 & 96.6 & 97.4 & 89.4 & 98.4 & 84.4 & 69.8 & 83.4 & 69.8 & 48.0 & 50.2 & 1.55 & 1.30 & 1.00 \\
Spatter & 97.8 & 97.8 & 98.4 & 98.0 & 97.6 & 96.8 & 93.6 & 88.0 & 79.6 & 91.8 & 92.2 & 76.8 & 1.72 & 1.58 & 1.54 \\
Contrast & 95.4 & 96.0 & 82.2 & 97.6 & 84.2 & 0.2 & 97.2 & 85.0 & 56.4 & 90.6 & 77.0 & 5.2 & 1.39 & 0.61 & 0.31 \\
Brightness & 96.6 & 97.2 & 96.4 & 97.6 & 97.2 & 96.6 & 97.4 & 97.4 & 97.4 & 90.6 & 90.8 & 91.6 & 1.44 & 1.10 & 0.91 \\
Saturate & 97.4 & 95.6 & 96.6 & 98.0 & 98.0 & 98.0 & 97.4 & 97.0 & 95.4 & 92.0 & 92.4 & 90.4 & 1.69 & 1.67 & 1.66 \\
JPEG Comp. & 96.4 & 94.4 & 89.6 & 98.2 & 98.6 & 97.6 & 95.6 & 88.0 & 90.6 & 93.0 & 90.6 & 84.6 & 1.60 & 1.55 & 1.54 \\
Pixelate & 94.6 & 94.4 & 93.6 & 98.0 & 96.0 & 95.6 & 97.8 & 95.0 & 94.0 & 91.0 & 84.4 & 78.4 & 1.57 & 1.48 & 1.58 \\
Elastic Trans. & 88.4 & 79.2 & 63.6 & 95.2 & 92.6 & 69.6 & 79.0 & 66.4 & 51.4 & 57.8 & 39.2 & 16.0 & 1.77 & 1.70 & 1.71 \\
\bottomrule
\end{tabular}
\end{table}

  \paragraph{Fused IB-Adapter-softmax.} Table~\ref{tab:detail_fusedib_adapter_softmax} presents results for a variant using softmax normalization instead of sigmoid in the fusion mechanism.

  % Detailed results for FusedIB-Adapter-softmax
% Auto-generated from CSV data
\begin{table}[t]
\centering
\setlength{\tabcolsep}{5pt}
\caption{Detailed results for Fused IB-Adapter-softmax on LIBERO and CALVIN benchmarks. We report success rate (\%) for LIBERO and average completed tasks for CALVIN.}
\label{tab:detail_fusedib_adapter_softmax}
\begin{tabular}{l ccc ccc ccc ccc ccc}
\toprule
 & \multicolumn{12}{c}{LIBERO} & \multicolumn{3}{c}{CALVIN} \\
\cmidrule(lr){2-13} \cmidrule(lr){14-16}
 & \multicolumn{3}{c}{Spatial} & \multicolumn{3}{c}{Object} & \multicolumn{3}{c}{Goal} & \multicolumn{3}{c}{Long} & \multicolumn{3}{c}{-} \\
\cmidrule(lr){2-4} \cmidrule(lr){5-7} \cmidrule(lr){8-10} \cmidrule(lr){11-13} \cmidrule(lr){14-16}
Corruption & S3 & S4 & S5 & S3 & S4 & S5 & S3 & S4 & S5 & S3 & S4 & S5 & S3 & S4 & S5 \\
\midrule
Clean & 72.2 & - & - & 96.0 & - & - & 97.2 & - & - & 93.2 & - & - & 0.46 & - & - \\
Gaussian Noise & 71.4 & 50.6 & 9.4 & 96.6 & 93.0 & 83.0 & 90.6 & 67.8 & 41.8 & 59.2 & 28.8 & 3.4 & 0.47 & 0.46 & 0.46 \\
Shot Noise & 65.0 & 34.0 & 6.0 & 95.8 & 90.2 & 85.6 & 90.4 & 66.2 & 45.6 & 60.4 & 20.6 & 2.6 & 0.45 & 0.47 & 0.45 \\
Impulse Noise & 68.6 & 50.0 & 11.8 & 97.8 & 93.4 & 87.0 & 90.6 & 66.0 & 44.8 & 62.0 & 29.2 & 4.2 & 0.47 & 0.46 & 0.46 \\
Speckle Noise & 70.2 & 55.8 & 36.8 & 97.2 & 96.2 & 90.4 & 93.2 & 89.6 & 75.0 & 71.8 & 56.2 & 29.4 & 0.47 & 0.47 & 0.46 \\
Gaussian Blur & 38.6 & 11.6 & 0.0 & 93.0 & 82.2 & 20.2 & 93.2 & 76.8 & 46.2 & 60.2 & 35.4 & 0.4 & 0.46 & 0.45 & 0.46 \\
Defocus Blur & 30.6 & 11.2 & 0.6 & 93.0 & 76.8 & 51.8 & 90.2 & 67.8 & 53.8 & 52.8 & 32.0 & 5.2 & 0.46 & 0.44 & 0.46 \\
Motion Blur & 49.0 & 21.8 & 6.8 & 93.6 & 69.0 & 20.2 & 92.8 & 59.2 & 39.0 & 56.4 & 10.4 & 0.2 & 0.46 & 0.46 & 0.45 \\
Zoom Blur & 29.4 & 19.8 & 7.8 & 48.0 & 5.8 & 18.0 & 80.8 & 73.0 & 56.0 & 28.8 & 10.0 & 1.4 & - & - & - \\
Fog & 67.0 & 55.6 & 25.6 & 97.8 & 98.6 & 98.6 & 95.2 & 93.2 & 75.4 & 81.2 & 66.8 & 17.8 & 0.47 & 0.46 & 0.46 \\
Frost & 58.4 & 52.4 & 44.8 & 85.0 & 80.8 & 68.0 & 71.8 & 65.8 & 54.4 & 34.0 & 29.4 & 13.0 & 0.44 & 0.47 & 0.45 \\
Snow & 53.0 & 47.6 & 52.2 & 96.2 & 85.0 & 94.8 & 86.2 & 66.6 & 80.6 & 58.8 & 28.0 & 20.4 & 0.46 & 0.47 & 0.45 \\
Spatter & 71.0 & 56.2 & 46.2 & 94.4 & 97.6 & 96.0 & 94.2 & 87.8 & 79.4 & 71.4 & 80.2 & 59.8 & 0.46 & 0.46 & 0.46 \\
Contrast & 73.0 & 55.6 & 6.0 & 97.6 & 98.2 & 4.2 & 97.6 & 95.6 & 64.6 & 85.0 & 68.0 & 8.0 & 0.46 & 0.46 & 0.47 \\
Brightness & 74.0 & 73.2 & 76.4 & 97.4 & 96.6 & 94.4 & 98.2 & 96.8 & 97.6 & 87.6 & 89.0 & 89.4 & 0.44 & 0.46 & 0.45 \\
Saturate & 71.8 & 70.6 & 64.6 & 98.0 & 96.6 & 96.4 & 95.6 & 97.0 & 97.2 & 91.4 & 88.6 & 84.8 & 0.46 & 0.45 & 0.46 \\
JPEG Comp. & 74.0 & 70.4 & 71.4 & 97.8 & 98.2 & 97.4 & 97.4 & 95.8 & 96.0 & 79.6 & 80.4 & 71.0 & 0.46 & 0.46 & 0.46 \\
Pixelate & 61.8 & 53.8 & 52.2 & 96.4 & 94.2 & 93.8 & 97.6 & 96.6 & 95.8 & 86.8 & 77.2 & 69.6 & 0.48 & 0.47 & 0.45 \\
Elastic Trans. & 30.6 & 19.4 & 11.8 & 94.2 & 91.6 & 68.2 & 68.0 & 40.8 & 14.4 & 47.0 & 19.8 & 0.4 & 0.45 & 0.45 & 0.44 \\
\bottomrule
\end{tabular}
\end{table}
