# Supplementary material for: Revisiting Chain-of-Thought Reasoning under Limited Supervision: Semi-supervised Chain-of-Thought Learning
Source: arXiv:2607.01511 source file (2026-07-01)
Supplement: Supplementary file 4 [file appendix_e.tex]

\section{Qualitative Results of Real-world Experiments}
\label{app:real_vis}

\begin{figure}[h]
    \centering
    \includegraphics[width=\linewidth]{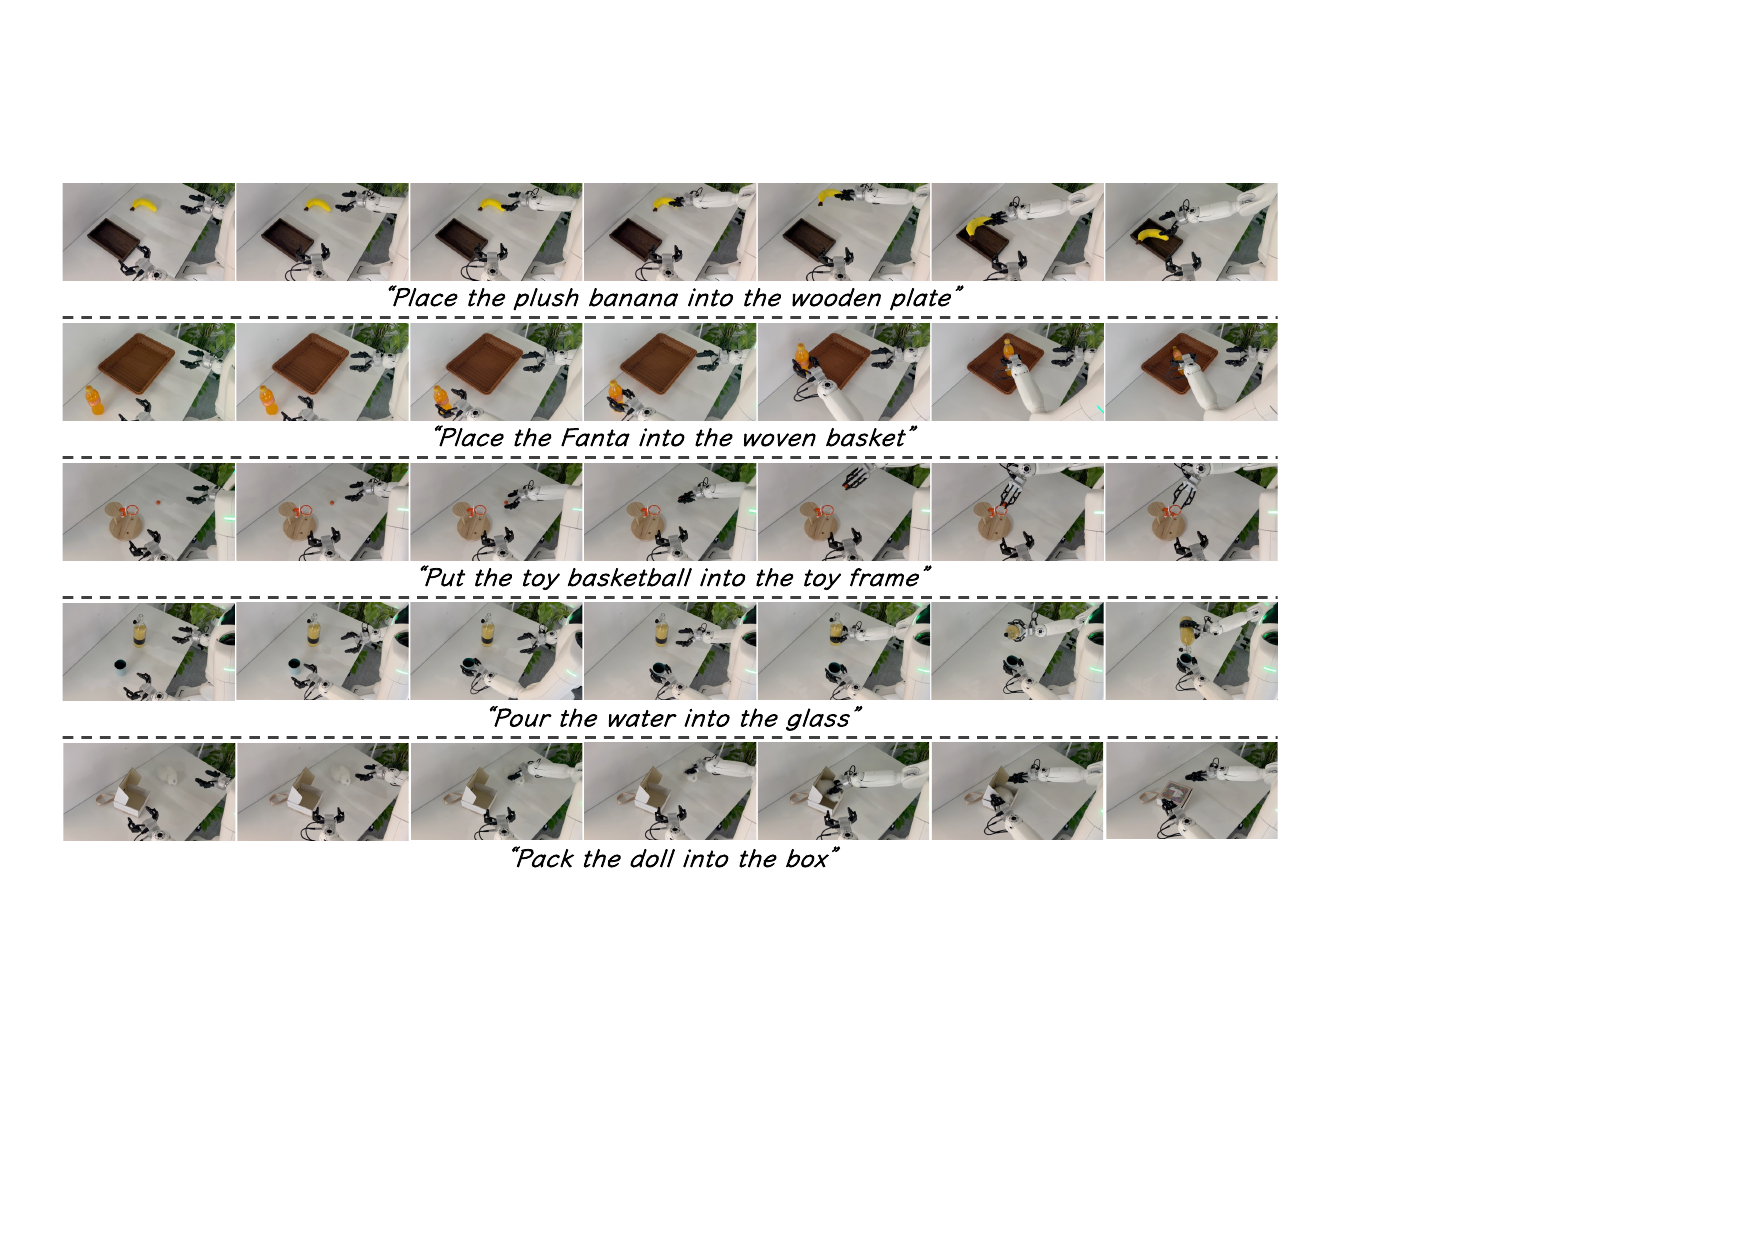}
    \caption{\textbf{Qualitative results of real-world experiments.} The figure displays successful execution sequences for five different manipulation tasks performed by the robot using StableVLA.}
    \label{fig:real_vis}
\end{figure}

\section{Detailed Related Work and Preliminaries}
\label{sec:detailed_related}

\subsection{Vision-Language-Action (VLA) Models}

Leveraging pre-trained Vision-Language Models (VLMs)~\cite{liu2023visual,comanici2025gemini,liu2024nvila,bai2025qwen2,zhu2025internvl3,xie2024show,li2024llava} for robotic control has emerged as a dominant paradigm in embodied intelligence~\citep{brohan2023rt-1, zitkovich2023rt-2, kim2024openvla, team2024octo}. However, pre-training these models from scratch relies on massive datasets, such as Open X-Embodiment~\citep{oneill2024open} and AgiBot~\cite{contributors2024agibotworldrepo}, requiring substantial computational resources. To mitigate this computational burden, VLA-Adapter~\citep{wang2025vla-adapter} proposes a resource-efficient alternative architecture. Diverging from standard paradigms, it bypasses the expensive pre-training stage on large-scale datasets, thereby directly transferring the general perceptual capabilities of VLMs to specific robotic domains.

Despite advances in training efficiency, a critical gap remains in \textit{architectural robustness}. In standard VLA models, the vision encoder~\citep{zhai2023sigmoid, oquab2023dinov2} is typically frozen during end-to-end training to preserve semantic priors~\citep{kim2024openvla, kim2025fine-tuning}, meaning input-level noise or corruption is propagated through the visual backbone. To align visual features with the downstream policy's action space, existing models use simple MLP projectors, which ideally act as the interface to suppress disturbances before they affect the policy network. Standard MLPs, while efficient at preserving spatial details, lack intrinsic mechanisms to filter out task-irrelevant nuisances. Our work addresses this by redesigning the projector's architecture to enable noise suppression during modality alignment.

\subsection{Robustness in Vision and Robotics}

Perceptual robustness is critical for the reliable deployment of robotic policies. In computer vision, this is typically evaluated using benchmarks such as ImageNet-C \cite{hendrycks2019robustness}, which introduces visual perturbations such as noise, blur, weather and digital corruptions. While classification tasks utilize the Mean Classification Error (mCE) as a standard metric, robustness in the VLA context is fundamentally tied to policy success rate under similar perturbations. Mainstream strategies to enhance robustness primarily rely on data-augmentation. In computer vision, techniques like ~\citep{hendrycks2021many} simulate corruptions during training to improve stability. Similarly, in robotic learning, Domain Randomization~\citep{tobin2017domain} is the standard approach, which randomly perturbs visual
textures or physical parameters in simulation.

However, these data-centric approaches face two significant limitations. First, they incur substantial training cost, often requiring models to be trained on vast augmented datasets. Second, these methods often rely on memorizing specific noise patterns, making it difficult to generalize to unseen corruption types. Therefore, we propose \textbf{StableVLA}, which focuses on intrinsic robustness through architectural design. We demonstrate that by reconstructing the modality alignment interface with the Information Bottleneck principle, VLA models can effectively filter visual perturbance without the need for exhaustive noise-pattern simulation.

\subsection{Attention Mechanism from the Perspective of Information Bottleneck}

Compared to CNNs, Vision Transformers (ViTs) exhibit superior robustness against various corruptions \citep{bai2021transformers, paul2022vision}. \citep{zhou2022understanding} attributes this property to the self-attention mechanism, which promotes \textit{visual grouping} where tokens aggregate into semantic clusters. This phenomenon is theoretically grounded in the Information Bottleneck (IB) principle \citep{tishby2000information}, which optimizes the trade-off between input compression and relevant information preservation. Notably, \citep{zhou2022understanding} proves that under Gaussian assumptions, the iterative optimization of the IB objective is mathematically equivalent to the self-attention operation.

While standard attention operates spatially, recent works explore visual grouping across channels. XCiT \citep{ali2021xcit} introduced Cross-Covariance Attention to compute channel-wise interactions, significantly reducing computational complexity. FAN \citep{zhou2022understanding} further establishes that this mechanism acts as subspace clustering; by applying the IB principle to the channel dimension, the model identifies coherent semantic subspaces while suppressing noisy channels. \textbf{StableVLA} extends this insight to VLA modality alignment, integrating a multi-head covariance mechanism to filter noisy channels and ensure robust semantic propagation for embodied decision-making.
