# Supplementary material for: Revisiting Chain-of-Thought Reasoning under Limited Supervision: Semi-supervised Chain-of-Thought Learning
Source: arXiv:2607.01511 source file (2026-07-01)
Supplement: Supplementary file 5 [file appendix_d.tex]

\clearpage
\section{Radar Chart Details}
  \label{app:radar}

  Figure~\ref{fig:radar} shows normalized robustness scores across 18 corruption types. For each corruption type, scores are averaged over clean images and severity levels 3--5, then normalized such that the best method equals 1. The corruption type indices are listed in Table~\ref{tab:corruption_index}.

  \begin{table}[h]
  \centering
  \caption{Corruption type indices for radar charts.}
  \label{tab:corruption_index}
  \begin{tabular}{cl|cl}
  \toprule
  Index & Corruption Type & Index & Corruption Type \\
  \midrule
  1 & Gaussian Noise & 10 & Frost \\
  2 & Shot Noise & 11 & Snow \\
  3 & Impulse Noise & 12 & Spatter \\
  4 & Speckle Noise & 13 & Contrast \\
  5 & Gaussian Blur & 14 & Brightness \\
  6 & Defocus Blur & 15 & Saturate \\
  7 & Motion Blur & 16 & JPEG Compression \\
  8 & Zoom Blur & 17 & Pixelate \\
  9 & Fog & 18 & Elastic Transform \\
  \bottomrule
  \multicolumn{4}{l}{\small *LIBERO-Spatial includes Glass Blur as index 19.}
  \end{tabular}
  \end{table}
