# Supplementary material for: Revisiting Chain-of-Thought Reasoning under Limited Supervision: Semi-supervised Chain-of-Thought Learning
Source: arXiv:2607.01511 source file (2026-07-01)
Supplement: Supplementary file 6 [file appendix_detail_fusedib_adapter_softmax.tex]

% Detailed results for FusedIB-Adapter-softmax
% Auto-generated from CSV data
\begin{table}[t]
\centering
\setlength{\tabcolsep}{5pt}
\caption{Detailed results for Fused IB-Adapter-softmax on LIBERO and CALVIN benchmarks. We report success rate (\%) for LIBERO and average completed tasks for CALVIN.}
\label{tab:detail_fusedib_adapter_softmax}
\begin{tabular}{l ccc ccc ccc ccc ccc}
\toprule
 & \multicolumn{12}{c}{LIBERO} & \multicolumn{3}{c}{CALVIN} \\
\cmidrule(lr){2-13} \cmidrule(lr){14-16}
 & \multicolumn{3}{c}{Spatial} & \multicolumn{3}{c}{Object} & \multicolumn{3}{c}{Goal} & \multicolumn{3}{c}{Long} & \multicolumn{3}{c}{-} \\
\cmidrule(lr){2-4} \cmidrule(lr){5-7} \cmidrule(lr){8-10} \cmidrule(lr){11-13} \cmidrule(lr){14-16}
Corruption & S3 & S4 & S5 & S3 & S4 & S5 & S3 & S4 & S5 & S3 & S4 & S5 & S3 & S4 & S5 \\
\midrule
Clean & 72.2 & - & - & 96.0 & - & - & 97.2 & - & - & 93.2 & - & - & 0.46 & - & - \\
Gaussian Noise & 71.4 & 50.6 & 9.4 & 96.6 & 93.0 & 83.0 & 90.6 & 67.8 & 41.8 & 59.2 & 28.8 & 3.4 & 0.47 & 0.46 & 0.46 \\
Shot Noise & 65.0 & 34.0 & 6.0 & 95.8 & 90.2 & 85.6 & 90.4 & 66.2 & 45.6 & 60.4 & 20.6 & 2.6 & 0.45 & 0.47 & 0.45 \\
Impulse Noise & 68.6 & 50.0 & 11.8 & 97.8 & 93.4 & 87.0 & 90.6 & 66.0 & 44.8 & 62.0 & 29.2 & 4.2 & 0.47 & 0.46 & 0.46 \\
Speckle Noise & 70.2 & 55.8 & 36.8 & 97.2 & 96.2 & 90.4 & 93.2 & 89.6 & 75.0 & 71.8 & 56.2 & 29.4 & 0.47 & 0.47 & 0.46 \\
Gaussian Blur & 38.6 & 11.6 & 0.0 & 93.0 & 82.2 & 20.2 & 93.2 & 76.8 & 46.2 & 60.2 & 35.4 & 0.4 & 0.46 & 0.45 & 0.46 \\
Defocus Blur & 30.6 & 11.2 & 0.6 & 93.0 & 76.8 & 51.8 & 90.2 & 67.8 & 53.8 & 52.8 & 32.0 & 5.2 & 0.46 & 0.44 & 0.46 \\
Motion Blur & 49.0 & 21.8 & 6.8 & 93.6 & 69.0 & 20.2 & 92.8 & 59.2 & 39.0 & 56.4 & 10.4 & 0.2 & 0.46 & 0.46 & 0.45 \\
Zoom Blur & 29.4 & 19.8 & 7.8 & 48.0 & 5.8 & 18.0 & 80.8 & 73.0 & 56.0 & 28.8 & 10.0 & 1.4 & - & - & - \\
Fog & 67.0 & 55.6 & 25.6 & 97.8 & 98.6 & 98.6 & 95.2 & 93.2 & 75.4 & 81.2 & 66.8 & 17.8 & 0.47 & 0.46 & 0.46 \\
Frost & 58.4 & 52.4 & 44.8 & 85.0 & 80.8 & 68.0 & 71.8 & 65.8 & 54.4 & 34.0 & 29.4 & 13.0 & 0.44 & 0.47 & 0.45 \\
Snow & 53.0 & 47.6 & 52.2 & 96.2 & 85.0 & 94.8 & 86.2 & 66.6 & 80.6 & 58.8 & 28.0 & 20.4 & 0.46 & 0.47 & 0.45 \\
Spatter & 71.0 & 56.2 & 46.2 & 94.4 & 97.6 & 96.0 & 94.2 & 87.8 & 79.4 & 71.4 & 80.2 & 59.8 & 0.46 & 0.46 & 0.46 \\
Contrast & 73.0 & 55.6 & 6.0 & 97.6 & 98.2 & 4.2 & 97.6 & 95.6 & 64.6 & 85.0 & 68.0 & 8.0 & 0.46 & 0.46 & 0.47 \\
Brightness & 74.0 & 73.2 & 76.4 & 97.4 & 96.6 & 94.4 & 98.2 & 96.8 & 97.6 & 87.6 & 89.0 & 89.4 & 0.44 & 0.46 & 0.45 \\
Saturate & 71.8 & 70.6 & 64.6 & 98.0 & 96.6 & 96.4 & 95.6 & 97.0 & 97.2 & 91.4 & 88.6 & 84.8 & 0.46 & 0.45 & 0.46 \\
JPEG Comp. & 74.0 & 70.4 & 71.4 & 97.8 & 98.2 & 97.4 & 97.4 & 95.8 & 96.0 & 79.6 & 80.4 & 71.0 & 0.46 & 0.46 & 0.46 \\
Pixelate & 61.8 & 53.8 & 52.2 & 96.4 & 94.2 & 93.8 & 97.6 & 96.6 & 95.8 & 86.8 & 77.2 & 69.6 & 0.48 & 0.47 & 0.45 \\
Elastic Trans. & 30.6 & 19.4 & 11.8 & 94.2 & 91.6 & 68.2 & 68.0 & 40.8 & 14.4 & 47.0 & 19.8 & 0.4 & 0.45 & 0.45 & 0.44 \\
\bottomrule
\end{tabular}
\end{table}
