# Supplementary material for: Revisiting Chain-of-Thought Reasoning under Limited Supervision: Semi-supervised Chain-of-Thought Learning
Source: arXiv:2607.01511 source file (2026-07-01)
Supplement: Supplementary file 7 [file appendix_detail_ib_adapter.tex]

% Detailed results for IB-Adapter
% Auto-generated from CSV data
\begin{table}[t]
\centering
\setlength{\tabcolsep}{5pt}
\caption{Detailed results for IB-Adapter on LIBERO and CALVIN benchmarks. We report success rate (\%) for LIBERO and average completed tasks for CALVIN.}
\label{tab:detail_ib_adapter}
\begin{tabular}{l ccc ccc ccc ccc ccc}
\toprule
 & \multicolumn{12}{c}{LIBERO} & \multicolumn{3}{c}{CALVIN} \\
\cmidrule(lr){2-13} \cmidrule(lr){14-16}
 & \multicolumn{3}{c}{Spatial} & \multicolumn{3}{c}{Object} & \multicolumn{3}{c}{Goal} & \multicolumn{3}{c}{Long} & \multicolumn{3}{c}{-} \\
\cmidrule(lr){2-4} \cmidrule(lr){5-7} \cmidrule(lr){8-10} \cmidrule(lr){11-13} \cmidrule(lr){14-16}
Corruption & S3 & S4 & S5 & S3 & S4 & S5 & S3 & S4 & S5 & S3 & S4 & S5 & S3 & S4 & S5 \\
\midrule
Clean & 97.8 & - & - & 0.97 & - & - & 97.4 & - & - & 93.8 & - & - & 1.64 & - & - \\
Gaussian Noise & 95.2 & 94.2 & 79.4 & 96.6 & 80.0 & 15.0 & 85.8 & 78.0 & 57.2 & 88.0 & 54.4 & 9.8 & 1.61 & 1.58 & 1.47 \\
Shot Noise & 96.0 & 91.4 & 76.6 & 95.4 & 67.8 & 15.0 & 86.4 & 70.6 & 62.6 & 84.8 & 56.2 & 1.7 & 1.63 & 1.61 & 1.43 \\
Impulse Noise & 97.4 & 95.0 & 84.0 & 97.4 & 86.2 & 23.4 & 89.0 & 77.0 & 55.4 & 87.0 & 54.8 & 12.4 & 1.66 & 1.60 & 1.50 \\
Speckle Noise & 96.8 & 96.2 & 91.4 & 96.6 & 97.0 & 92.2 & 84.2 & 84.2 & 77.2 & 89.4 & 80.0 & 58.4 & 1.55 & 1.54 & 1.37 \\
Gaussian Blur & 88.6 & 80.8 & 32.4 & 88.0 & 36.6 & 2.0 & 93.6 & 86.0 & 68.4 & 56.0 & 41.2 & 5.2 & 1.52 & 1.44 & 1.26 \\
Glass Blur & 89.4 & 75.4 & 43.2 & - & - & - & - & - & - & - & - & - & - & - & - \\
Defocus Blur & 88.0 & 78.6 & 45.4 & 85.2 & 35.6 & 17.4 & 89.2 & 79.6 & 68.4 & 50.6 & 37.4 & 13.6 & 1.53 & 1.46 & 1.32 \\
Motion Blur & 93.0 & 87.6 & 74.6 & 91.4 & 40.6 & 2.0 & 91.2 & 75.2 & 56.0 & 71.0 & 21.0 & 1.8 & 1.44 & 1.23 & 1.16 \\
Zoom Blur & 96.0 & 90.4 & 88.0 & 50.4 & 13.2 & 12.0 & 92.6 & 83.4 & 66.6 & 44.0 & 18.5 & 10.4 & 1.54 & 1.59 & 1.48 \\
Fog & 98.4 & 98.0 & 93.4 & 96.4 & 96.4 & 56.8 & 86.6 & 86.0 & 65.4 & 87.6 & 81.4 & 52.2 & 1.11 & 1.09 & 0.92 \\
Frost & 95.2 & 93.8 & 89.4 & 94.0 & 85.8 & 69.8 & 75.0 & 70.4 & 63.0 & 68.8 & 60.8 & 43.2 & 1.70 & 1.66 & 1.61 \\
Snow & 98.8 & 97.4 & 96.6 & 97.4 & 89.4 & 98.4 & 84.4 & 69.8 & 83.4 & 69.8 & 48.0 & 50.2 & 1.55 & 1.30 & 1.00 \\
Spatter & 97.8 & 97.8 & 98.4 & 98.0 & 97.6 & 96.8 & 93.6 & 88.0 & 79.6 & 91.8 & 92.2 & 76.8 & 1.72 & 1.58 & 1.54 \\
Contrast & 95.4 & 96.0 & 82.2 & 97.6 & 84.2 & 0.2 & 97.2 & 85.0 & 56.4 & 90.6 & 77.0 & 5.2 & 1.39 & 0.61 & 0.31 \\
Brightness & 96.6 & 97.2 & 96.4 & 97.6 & 97.2 & 96.6 & 97.4 & 97.4 & 97.4 & 90.6 & 90.8 & 91.6 & 1.44 & 1.10 & 0.91 \\
Saturate & 97.4 & 95.6 & 96.6 & 98.0 & 98.0 & 98.0 & 97.4 & 97.0 & 95.4 & 92.0 & 92.4 & 90.4 & 1.69 & 1.67 & 1.66 \\
JPEG Comp. & 96.4 & 94.4 & 89.6 & 98.2 & 98.6 & 97.6 & 95.6 & 88.0 & 90.6 & 93.0 & 90.6 & 84.6 & 1.60 & 1.55 & 1.54 \\
Pixelate & 94.6 & 94.4 & 93.6 & 98.0 & 96.0 & 95.6 & 97.8 & 95.0 & 94.0 & 91.0 & 84.4 & 78.4 & 1.57 & 1.48 & 1.58 \\
Elastic Trans. & 88.4 & 79.2 & 63.6 & 95.2 & 92.6 & 69.6 & 79.0 & 66.4 & 51.4 & 57.8 & 39.2 & 16.0 & 1.77 & 1.70 & 1.71 \\
\bottomrule
\end{tabular}
\end{table}
