# Supplementary material for: Revisiting Chain-of-Thought Reasoning under Limited Supervision: Semi-supervised Chain-of-Thought Learning
Source: arXiv:2607.01511 source file (2026-07-01)
Supplement: Supplementary file 8 [file appendix_detail_openpi.tex]

% Detailed results for OpenPI
% Auto-generated from CSV data
\begin{table}[t]
\centering
\setlength{\tabcolsep}{6pt}
\caption{Detailed results for OpenPI on LIBERO benchmark. We report success rate (\%).}
\label{tab:detail_openpi}
\begin{tabular}{l ccc ccc ccc ccc}
\toprule
 & \multicolumn{3}{c}{Spatial} & \multicolumn{3}{c}{Object} & \multicolumn{3}{c}{Goal} & \multicolumn{3}{c}{Long} \\
\cmidrule(lr){2-4} \cmidrule(lr){5-7} \cmidrule(lr){8-10} \cmidrule(lr){11-13}
Corruption & S3 & S4 & S5 & S3 & S4 & S5 & S3 & S4 & S5 & S3 & S4 & S5 \\
\midrule
Clean & 98.4 & - & - & 99.4 & - & - & 97.2 & - & - & 92.0 & - & - \\
Gaussian Noise & 98.4 & 92.0 & 29.8 & 98.4 & 98.0 & 58.4 & 96.2 & 78.0 & 21.6 & 88.4 & 73.2 & 13.0 \\
Shot Noise & 98.0 & 75.0 & 24.2 & 98.8 & 95.8 & 53.0 & 94.0 & 79.6 & 31.8 & 89.4 & 72.6 & 29.8 \\
Impulse Noise & 98.4 & 94.8 & 36.0 & 99.4 & 98.6 & 62.0 & 95.2 & 79.4 & 28.2 & 90.0 & 73.4 & 17.6 \\
Speckle Noise & 97.6 & 98.0 & 77.8 & 98.4 & 98.6 & 96.6 & 96.6 & 92.6 & 86.6 & 87.0 & 83.6 & 79.0 \\
Gaussian Blur & 41.4 & 10.8 & 0.0 & 88.8 & 10.0 & 0.0 & 76.4 & 44.6 & 1.6 & 11.0 & 0.4 & 0.0 \\
Glass Blur & 59.8 & 39.2 & 9.0 & - & - & - & - & - & - & - & - & - \\
Defocus Blur & 43.2 & 17.6 & 6.8 & 83.0 & 32.4 & 0.8 & 69.2 & 47.2 & 11.6 & 10.6 & 0.6 & 0.0 \\
Motion Blur & 81.6 & 38.4 & 10.8 & 96.2 & 77.8 & 34.8 & 87.0 & 55.0 & 24.4 & 62.4 & 21.6 & 1.2 \\
Zoom Blur & 80.4 & 75.8 & 74.4 & 99.4 & 98.4 & 97.4 & 89.6 & 83.2 & 77.0 & 60.0 & 0.8 & 1.0 \\
Fog & 96.8 & 92.0 & 81.0 & 98.4 & 99.0 & 97.2 & 97.0 & 96.0 & 82.4 & 87.6 & 76.4 & 50.2 \\
Frost & 95.8 & 91.0 & 77.4 & 98.8 & 98.8 & 95.4 & 85.8 & 81.6 & 72.4 & 47.6 & 74.2 & 56.2 \\
Snow & 97.2 & 91.8 & 91.4 & 99.4 & 98.2 & 98.2 & 92.8 & 77.8 & 79.8 & 89.6 & 76.0 & 40.8 \\
Spatter & 99.0 & 98.0 & 96.0 & 98.6 & 99.6 & 99.4 & 96.8 & 96.8 & 93.0 & 94.0 & 93.6 & 90.0 \\
Contrast & 98.4 & 97.0 & 94.0 & 98.6 & 99.0 & 96.0 & 98.0 & 97.2 & 93.6 & 89.6 & 88.6 & 67.4 \\
Brightness & 98.2 & 98.2 & 98.0 & 98.8 & 99.2 & 99.4 & 8.2 & 97.2 & 97.0 & 92.2 & 91.8 & 93.2 \\
Saturate & 99.2 & 99.0 & 98.4 & 97.6 & 98.2 & 98.8 & 98.4 & 97.0 & 97.2 & 92.8 & 92.2 & 94.0 \\
JPEG Comp. & 96.0 & 97.2 & 96.8 & 98.4 & 99.2 & 99.0 & 96.2 & 95.0 & 95.8 & 88.6 & 88.2 & 88.2 \\
Pixelate & 99.4 & 96.8 & 88.2 & 98.0 & 90.4 & 88.0 & 97.4 & 96.4 & 80.6 & 93.6 & 83.4 & 55.8 \\
Elastic Trans. & 99.2 & 97.8 & 96.0 & 99.6 & 99.8 & 100.0 & 94.8 & 90.4 & 81.4 & 95.0 & 90.0 & 81.6 \\
\bottomrule
\end{tabular}
\end{table}
