# Supplementary material for: Revisiting Chain-of-Thought Reasoning under Limited Supervision: Semi-supervised Chain-of-Thought Learning
Source: arXiv:2607.01511 source file (2026-07-01)
Supplement: Supplementary file 9 [file appendix_detail_openvla.tex]

% Detailed results for OpenVLA
% Auto-generated from CSV data
\begin{table}[t]
\centering
\setlength{\tabcolsep}{6pt}
\caption{Detailed results for OpenVLA on LIBERO benchmark. We report success rate (\%).}
\label{tab:detail_openvla}
\begin{tabular}{l ccc ccc ccc ccc}
\toprule
 & \multicolumn{3}{c}{Spatial} & \multicolumn{3}{c}{Object} & \multicolumn{3}{c}{Goal} & \multicolumn{3}{c}{Long} \\
\cmidrule(lr){2-4} \cmidrule(lr){5-7} \cmidrule(lr){8-10} \cmidrule(lr){11-13}
Corruption & S3 & S4 & S5 & S3 & S4 & S5 & S3 & S4 & S5 & S3 & S4 & S5 \\
\midrule
Clean & 80.0 & - & - & 69.6 & - & - & 74.0 & - & - & 55.5 & - & - \\
Gaussian Noise & 50.2 & 0.6 & 0.0 & 0.6 & 0.0 & 0.0 & 31.4 & 4.8 & 0.0 & 8.4 & 0.2 & 0.0 \\
Shot Noise & 39.0 & 0.0 & 0.0 & 0.4 & 0.0 & 0.0 & 23.6 & 2.8 & 0.0 & 5.6 & 0.0 & 0.0 \\
Impulse Noise & 55.2 & 1.4 & 0.0 & 3.0 & 0.0 & 0.0 & 41.0 & 4.8 & 0.0 & 9.2 & 1.6 & 0.0 \\
Speckle Noise & 61.0 & 26.0 & 2.8 & 5.2 & 0.2 & 0.0 & 40.8 & 17.2 & 8.4 & 17.6 & 3.8 & 0.0 \\
Gaussian Blur & 0.0 & 0.0 & 0.0 & 0.0 & 0.0 & 0.0 & 2.4 & 0.2 & 0.0 & 0.0 & 0.0 & 0.0 \\
Glass Blur & 0.0 & 0.0 & 0.0 & - & - & - & - & - & - & - & - & - \\
Defocus Blur & 0.0 & 0.0 & 0.0 & 0.0 & 0.0 & 0.0 & 0.4 & 0.2 & 0.8 & 0.0 & 0.0 & 0.0 \\
Motion Blur & 0.0 & 0.0 & 0.0 & 0.0 & 0.0 & 0.0 & 0.6 & 0.0 & 0.0 & 0.0 & 0.0 & 0.0 \\
Zoom Blur & 7.6 & 3.2 & 0.2 & 0.6 & 0.0 & 0.0 & 14.0 & 3.4 & 1.6 & 3.0 & 0.2 & 0.0 \\
Fog & 74.6 & 69.4 & 38.0 & 46.4 & 24.2 & 0.4 & 76.2 & 69.0 & 40.2 & 51.0 & 46.4 & 20.2 \\
Frost & 20.2 & 16.8 & 4.4 & 0.6 & 0.2 & 0.4 & 28.4 & 22.8 & 14.0 & 15.6 & 12.0 & 4.2 \\
Snow & 39.0 & 10.4 & 22.2 & 0.4 & 0.0 & 0.0 & 28.6 & 19.8 & 15.0 & 14.6 & 2.2 & 3.2 \\
Spatter & 65.4 & 32.4 & 3.8 & 14.2 & 0.2 & 0.0 & 50.2 & 37.0 & 16.2 & 36.0 & 12.6 & 2.2 \\
Contrast & 71.2 & 52.6 & 6.8 & 57.4 & 28.0 & 0.0 & 75.0 & 69.2 & 16.8 & 50.2 & 38.8 & 10.0 \\
Brightness & 78.4 & 73.8 & 62.8 & 64.6 & 53.2 & 29.0 & 76.0 & 73.4 & 60.8 & 52.6 & 45.6 & 41.2 \\
Saturate & 80.8 & 81.4 & 74.2 & 65.8 & 47.8 & 12.6 & 75.2 & 75.2 & 69.8 & 55.6 & 48.6 & 40.2 \\
JPEG Comp. & 72.4 & 69.8 & 56.6 & 42.6 & 29.4 & 5.8 & 73.8 & 63.2 & 45.0 & 31.8 & 10.0 & 4.2 \\
Pixelate & 60.0 & 29.0 & 7.2 & 24.8 & 3.6 & 0.0 & 53.6 & 21.2 & 5.2 & 15.4 & 1.0 & 0.0 \\
Elastic Trans. & 2.6 & 0.2 & 0.0 & 1.0 & 0.2 & 0.0 & 5.4 & 1.8 & 0.4 & 3.2 & 1.0 & 0.0 \\
\bottomrule
\end{tabular}
\end{table}
