# Supplementary material for: Revisiting Chain-of-Thought Reasoning under Limited Supervision: Semi-supervised Chain-of-Thought Learning
Source: arXiv:2607.01511 source file (2026-07-01)
Supplement: Supplementary file 10 [file appendix_detail_openvla_oft.tex]

% Detailed results for OpenVLA-OFT
% Auto-generated from CSV data
\begin{table}[t]
\centering
\setlength{\tabcolsep}{6pt}
\caption{Detailed results for OpenVLA-OFT on LIBERO benchmark. We report success rate (\%).}
\label{tab:detail_openvla_oft}
\begin{tabular}{l ccc ccc ccc ccc}
\toprule
 & \multicolumn{3}{c}{Spatial} & \multicolumn{3}{c}{Object} & \multicolumn{3}{c}{Goal} & \multicolumn{3}{c}{Long} \\
\cmidrule(lr){2-4} \cmidrule(lr){5-7} \cmidrule(lr){8-10} \cmidrule(lr){11-13}
Corruption & S3 & S4 & S5 & S3 & S4 & S5 & S3 & S4 & S5 & S3 & S4 & S5 \\
\midrule
Clean & 92.6 & - & - & 98.4 & - & - & 96.8 & - & - & 94.4 & - & - \\
Gaussian Noise & 90.4 & 89.2 & 67.8 & 88.6 & 56.4 & 21.2 & 94.4 & 87.2 & 56.0 & 74.6 & 47.6 & 13.8 \\
Shot Noise & 90.8 & 85.4 & 70.2 & 88.0 & 85.4 & 70.2 & 97.0 & 76.0 & 57.4 & 82.4 & 45.6 & 12.0 \\
Impulse Noise & 90.2 & 85.6 & 64.8 & 90.2 & 56.0 & 25.8 & 95.6 & 84.0 & 56.4 & 80.2 & 48.0 & 18.8 \\
Speckle Noise & 92.4 & 90.0 & 84.4 & 91.4 & 83.6 & 56.8 & 96.6 & 94.2 & 80.8 & 88.4 & 81.0 & 47.0 \\
Gaussian Blur & 86.8 & 80.6 & 46.6 & 53.0 & 35.0 & 4.6 & 96.4 & 84.8 & 48.0 & 78.0 & 38.4 & 6.2 \\
Glass Blur & 84.4 & 73.6 & 42.6 & - & - & - & - & - & - & - & - & - \\
Defocus Blur & 85.6 & 69.4 & 46.8 & 47.6 & 27.6 & 11.2 & 93.0 & 76.8 & 53.4 & 57.8 & 30.2 & 11.0 \\
Motion Blur & 77.6 & 55.6 & 39.4 & 57.4 & 20.6 & 3.8 & 89.6 & 51.6 & 27.8 & 42.6 & 16.0 & 4.6 \\
Zoom Blur & 82.2 & 71.8 & 62.6 & 70.8 & 44.0 & 30.8 & 87.4 & 77.6 & 69.6 & 54.8 & 38.2 & 13.4 \\
Fog & 90.4 & 87.8 & 73.0 & 94.0 & 85.6 & 59.2 & 96.0 & 92.0 & 63.0 & 81.6 & 71.0 & 37.8 \\
Frost & 91.6 & 89.0 & 83.0 & 84.0 & 80.8 & 83.0 & 90.6 & 83.8 & 70.2 & 69.2 & 61.4 & 54.2 \\
Snow & 92.4 & 89.2 & 93.0 & 88.2 & 80.2 & 61.4 & 89.6 & 64.6 & 83.0 & 61.6 & 35.2 & 29.0 \\
Spatter & 93.2 & 90.0 & 84.0 & 96.6 & 92.6 & 86.4 & 95.4 & 90.8 & 84.6 & 88.6 & 90.8 & 71.8 \\
Contrast & 91.8 & 89.4 & 69.6 & 96.0 & 90.6 & 56.8 & 98.4 & 93.2 & 66.2 & 91.0 & 84.6 & 32.4 \\
Brightness & 93.8 & 94.2 & 92.4 & 96.0 & 94.8 & 93.0 & 99.0 & 98.2 & 97.6 & 91.2 & 91.8 & 90.0 \\
Saturate & 92.8 & 92.4 & 92.8 & 92.8 & 95.4 & 94.0 & 95.4 & 95.0 & 97.6 & 91.6 & 91.8 & 85.2 \\
JPEG Comp. & 92.2 & 92.2 & 92.6 & 97.0 & 96.8 & 91.8 & 98.6 & 96.0 & 97.2 & 92.0 & 87.4 & 83.8 \\
Pixelate & 91.6 & 90.8 & 90.4 & 86.2 & 69.6 & 64.2 & 97.0 & 97.4 & 96.6 & 91.8 & 90.0 & 84.6 \\
Elastic Trans. & 86.6 & 80.2 & 74.4 & 66.6 & 51.2 & 36.0 & 90.6 & 79.8 & 60.2 & 80.0 & 65.2 & 29.6 \\
\bottomrule
\end{tabular}
\end{table}
