# Supplementary material for: Revisiting Chain-of-Thought Reasoning under Limited Supervision: Semi-supervised Chain-of-Thought Learning
Source: arXiv:2607.01511 source file (2026-07-01)
Supplement: Supplementary file 11 [file appendix_detail_stablevla.tex]

% Detailed results for StableVLA
% Auto-generated from CSV data
\begin{table}[h]
\centering
\setlength{\tabcolsep}{5pt}
\caption{Detailed results for StableVLA on LIBERO and CALVIN benchmarks. We report success rate (\%) for LIBERO and average completed tasks for CALVIN.}
\label{tab:detail_stablevla}
\begin{tabular}{l ccc ccc ccc ccc ccc}
\toprule
 & \multicolumn{12}{c}{LIBERO} & \multicolumn{3}{c}{CALVIN} \\
\cmidrule(lr){2-13} \cmidrule(lr){14-16}
 & \multicolumn{3}{c}{Spatial} & \multicolumn{3}{c}{Object} & \multicolumn{3}{c}{Goal} & \multicolumn{3}{c}{Long} & \multicolumn{3}{c}{-} \\
\cmidrule(lr){2-4} \cmidrule(lr){5-7} \cmidrule(lr){8-10} \cmidrule(lr){11-13} \cmidrule(lr){14-16}
Corruption & S3 & S4 & S5 & S3 & S4 & S5 & S3 & S4 & S5 & S3 & S4 & S5 & S3 & S4 & S5 \\
\midrule
Clean & 96.2 & - & - & 98.8 & - & - & 98.0 & - & - & 93.6 & - & - & 4.17 & - & - \\
Gaussian Noise & 96.0 & 92.8 & 74.0 & 95.4 & 85.0 & 64.8 & 95.2 & 85.2 & 53.2 & 82.8 & 53.6 & 25.0 & 2.02 & 1.26 & 0.60 \\
Shot Noise & 95.4 & 88.0 & 71.0 & 93.2 & 80.6 & 64.0 & 96.2 & 81.4 & 61.8 & 84.8 & 63.0 & 23.4 & 1.85 & 0.82 & 0.46 \\
Impulse Noise & 94.6 & 93.2 & 80.8 & 96.0 & 83.2 & 62.8 & 96.2 & 81.8 & 57.2 & 81.2 & 55.2 & 30.2 & 2.60 & 1.32 & 0.72 \\
Speckle Noise & 94.6 & 96.6 & 90.4 & 95.6 & 93.2 & 87.2 & 97.8 & 96.0 & 86.4 & 87.2 & 84.0 & 71.8 & 2.16 & 1.49 & 0.90 \\
Gaussian Blur & 91.6 & 83.0 & 49.4 & 84.4 & 45.4 & 2.4 & 91.8 & 74.0 & 42.6 & 55.4 & 31.2 & 2.8 & 2.18 & 0.94 & 0.34 \\
Glass Blur & 91.2 & 83.6 & 55.8 & - & - & - & - & - & - & - & - & - & - & - & - \\
Defocus Blur & 89.4 & 81.6 & 65.0 & 72.8 & 46.8 & 24.8 & 85.8 & 63.0 & 47.2 & 49.6 & 27.2 & 10.6 & 1.56 & 0.64 & 0.34 \\
Motion Blur & 89.6 & 90.4 & 82.6 & 98.2 & 72.0 & 27.4 & 93.4 & 59.8 & 37.6 & 66.0 & 21.6 & 1.0 & 1.23 & 0.46 & 0.24 \\
Zoom Blur & 95.8 & 93.6 & 86.2 & 60.8 & 49.8 & 46.8 & 91.0 & 82.8 & 69.0 & 36.8 & 16.8 & 11.2 & 3.48 & 2.86 & 2.10 \\
Fog & 95.0 & 94.0 & 94.4 & 99.8 & 99.6 & 94.8 & 94.4 & 95.2 & 81.4 & 78.4 & 75.0 & 57.0 & 2.84 & 1.97 & 0.88 \\
Frost & 96.0 & 93.8 & 89.8 & 84.0 & 79.4 & 67.4 & 92.0 & 88.6 & 81.0 & 72.6 & 69.2 & 54.8 & 3.11 & 2.99 & 2.64 \\
Snow & 95.4 & 94.8 & 94.2 & 97.4 & 92.2 & 95.4 & 92.0 & 85.4 & 95.4 & 61.0 & 39.2 & 33.0 & 3.45 & 2.50 & 1.62 \\
Spatter & 96.6 & 95.0 & 95.2 & 98.2 & 98.6 & 93.4 & 93.8 & 94.4 & 91.2 & 90.8 & 94.4 & 87.2 & 4.13 & 4.04 & 3.74 \\
Contrast & 94.2 & 95.2 & 68.0 & 99.0 & 98.4 & 78.6 & 97.6 & 95.6 & 56.8 & 93.6 & 90.2 & 52.6 & 3.74 & 2.30 & 0.59 \\
Brightness & 96.4 & 96.2 & 97.0 & 98.4 & 99.0 & 98.4 & 98.0 & 99.0 & 98.0 & 92.4 & 90.2 & 90.6 & 4.04 & 3.48 & 2.71 \\
Saturate & 96.6 & 96.4 & 98.0 & 98.8 & 98.2 & 97.2 & 96.6 & 98.2 & 97.8 & 93.4 & 92.0 & 89.8 & 4.20 & 4.19 & 4.17 \\
JPEG Comp. & 96.2 & 96.6 & 94.4 & 98.6 & 98.8 & 97.4 & 96.8 & 97.4 & 96.8 & 89.4 & 88.8 & 73.8 & 2.79 & 2.42 & 1.50 \\
Pixelate & 94.6 & 95.2 & 94.4 & 96.4 & 96.4 & 95.6 & 97.6 & 96.8 & 95.6 & 92.8 & 93.0 & 84.6 & 2.60 & 2.86 & 2.69 \\
Elastic Trans. & 91.6 & 90.4 & 78.2 & 95.6 & 89.0 & 65.8 & 74.4 & 55.2 & 45.2 & 65.2 & 38.8 & 16.2 & 1.94 & 1.49 & 0.99 \\
\bottomrule
\end{tabular}
\end{table}
