# Supplementary material for: Revisiting Chain-of-Thought Reasoning under Limited Supervision: Semi-supervised Chain-of-Thought Learning
Source: arXiv:2607.01511 source file (2026-07-01)
Supplement: Supplementary file 12 [file appendix_detail_vla_adapter_pro.tex]

% Detailed results for VLA-Adapter-Pro
% Auto-generated from CSV data
\begin{table}[h]
\centering
\setlength{\tabcolsep}{5pt}
\caption{Detailed results for VLA-Adapter-Pro on LIBERO and CALVIN benchmarks. We report success rate (\%) for LIBERO and average completed tasks for CALVIN.}
\label{tab:detail_vla_adapter_pro}
\begin{tabular}{l ccc ccc ccc ccc ccc}
\toprule
 & \multicolumn{12}{c}{LIBERO} & \multicolumn{3}{c}{CALVIN} \\
\cmidrule(lr){2-13} \cmidrule(lr){14-16}
 & \multicolumn{3}{c}{Spatial} & \multicolumn{3}{c}{Object} & \multicolumn{3}{c}{Goal} & \multicolumn{3}{c}{Long} & \multicolumn{3}{c}{-} \\
\cmidrule(lr){2-4} \cmidrule(lr){5-7} \cmidrule(lr){8-10} \cmidrule(lr){11-13} \cmidrule(lr){14-16}
Corruption & S3 & S4 & S5 & S3 & S4 & S5 & S3 & S4 & S5 & S3 & S4 & S5 & S3 & S4 & S5 \\
\midrule
Clean & 96.0 & - & - & 96.8 & - & - & 97.4 & - & - & 94.4 & - & - & 4.14 & - & - \\
Gaussian Noise & 98.2 & 93.8 & 32.4 & 97.2 & 53.8 & 0.0 & 79.4 & 53.4 & 26.0 & 69.4 & 37.0 & 1.0 & 2.35 & 1.03 & 0.29 \\
Shot Noise & 97.8 & 84.6 & 12.8 & 93.8 & 23.4 & 0.0 & 74.6 & 49.2 & 36.6 & 76.4 & 22.8 & 4.0 & 2.06 & 0.80 & 0.21 \\
Impulse Noise & 99.0 & 93.2 & 38.0 & 98.8 & 67.8 & 0.0 & 77.4 & 56.8 & 26.4 & 72.0 & 38.6 & 2.6 & 2.92 & 1.14 & 0.37 \\
Speckle Noise & 97.8 & 97.4 & 85.0 & 97.2 & 85.4 & 40.0 & 75.2 & 67.8 & 54.6 & 83.2 & 71.2 & 28.2 & 2.59 & 1.76 & 0.90 \\
Gaussian Blur & 89.2 & 56.2 & 3.8 & 28.0 & 0.0 & 0.0 & 87.6 & 72.6 & 26.8 & 37.0 & 3.2 & 0.0 & 0.76 & 0.12 & 0.00 \\
Glass Blur & 72.6 & 41.4 & 8.0 & - & - & - & - & - & - & - & - & - & - & - & - \\
Defocus Blur & 77.8 & 35.6 & 6.6 & 5.0 & 0.0 & 0.0 & 81.6 & 60.0 & 36.4 & 19.6 & 1.4 & 0.0 & 0.41 & 0.06 & 0.00 \\
Motion Blur & 88.0 & 59.2 & 29.0 & 11.6 & 0.0 & 0.0 & 89.2 & 47.2 & 21.4 & 36.2 & 8.0 & 0.0 & 0.69 & 0.08 & 0.01 \\
Zoom Blur & 87.8 & 78.0 & 71.8 & 19.2 & 6.0 & 0.0 & 73.2 & 59.0 & 41.0 & 9.0 & 1.2 & 2.0 & 2.95 & 2.43 & 1.76 \\
Fog & 98.6 & 98.0 & 93.6 & 63.4 & 11.8 & 0.2 & 77.4 & 71.0 & 46.2 & 52.4 & 37.0 & 12.6 & 2.77 & 2.38 & 1.34 \\
Frost & 93.8 & 90.2 & 81.4 & 32.2 & 22.8 & 8.2 & 59.8 & 55.0 & 43.2 & 49.4 & 36.4 & 19.0 & 3.61 & 3.46 & 3.37 \\
Snow & 97.2 & 91.6 & 95.6 & 63.0 & 7.6 & 59.2 & 58.2 & 40.6 & 57.0 & 41.8 & 6.0 & 13.6 & 3.64 & 3.03 & 2.73 \\
Spatter & 98.4 & 96.6 & 88.0 & 97.2 & 53.4 & 6.0 & 89.2 & 77.6 & 61.0 & 82.4 & 68.2 & 36.2 & 4.05 & 3.93 & 3.23 \\
Contrast & 99.4 & 97.8 & 25.8 & 88.6 & 0.0 & 0.0 & 91.4 & 79.0 & 26.0 & 68.6 & 4.4 & 0.0 & 2.54 & 0.78 & 0.01 \\
Brightness & 98.2 & 99.4 & 97.8 & 98.8 & 98.4 & 98.6 & 89.8 & 89.6 & 88.2 & 91.2 & 91.4 & 86.0 & 4.16 & 4.12 & 3.74 \\
Saturate & 99.2 & 99.2 & 99.2 & 98.4 & 98.4 & 94.0 & 98.0 & 92.8 & 88.0 & 93.8 & 80.8 & 84.0 & 4.13 & 4.13 & 4.14 \\
JPEG Comp. & 99.0 & 98.2 & 98.6 & 98.4 & 98.8 & 98.8 & 87.4 & 84.4 & 81.6 & 90.4 & 88.8 & 81.4 & 1.80 & 1.14 & 0.53 \\
Pixelate & 98.2 & 97.2 & 94.8 & 96.2 & 91.0 & 80.0 & 97.0 & 95.0 & 88.6 & 89.6 & 85.0 & 69.4 & 2.65 & 2.01 & 1.94 \\
Elastic Trans. & 90.2 & 74.8 & 50.2 & 90.8 & 75.0 & 42.6 & 44.2 & 14.2 & 2.8 & 80.4 & 56.8 & 31.8 & 1.89 & 1.61 & 1.26 \\
\bottomrule
\end{tabular}
\end{table}
