# Supplementary material for: Revisiting Chain-of-Thought Reasoning under Limited Supervision: Semi-supervised Chain-of-Thought Learning
Source: arXiv:2607.01511 source file (2026-07-01)
Supplement: Supplementary file 13 [file appendix_table1_full_libero.tex]

% Appendix Table: Full comparison on LIBERO benchmark (grouped by training paradigm)
% Auto-generated from CSV data
\begin{table}[h]
\centering
\setlength{\tabcolsep}{3.5pt}
\footnotesize
\caption{Full comparison on LIBERO benchmark. Methods are grouped by training paradigm. We report success rate (\%). \textbf{Bold}: best, \underline{underline}: second best.}
\label{tab:app_full_libero}
\begin{tabular}{p{1.2cm}l cccc cccc cccc cccc}
\toprule
 & & \multicolumn{4}{c}{Spatial} & \multicolumn{4}{c}{Object} & \multicolumn{4}{c}{Goal} & \multicolumn{4}{c}{Long} \\
\cmidrule(lr){3-6} \cmidrule(lr){7-10} \cmidrule(lr){11-14} \cmidrule(lr){15-18}
Training & Method & C & S3 & S4 & S5 & C & S3 & S4 & S5 & C & S3 & S4 & S5 & C & S3 & S4 & S5 \\
\midrule
\multirow{2}{1.2cm}{\raggedright\scriptsize OpenX\\Pretrain} & OpenVLA & 80.0 & 40.9 & 24.6 & 14.7 & 69.6 & 18.2 & 10.4 & 2.7 & 74.0 & 38.7 & 27.0 & 16.3 & 55.5 & 20.5 & 12.4 & 7.0 \\
 & OpenVLA-OFT & 92.6 & 89.3 & \underline{84.0} & \underline{72.1} & 98.4 & 82.5 & 69.2 & 52.8 & 96.8 & \textbf{94.5} & \underline{84.6} & \underline{70.3} & \textbf{94.4} & \textbf{77.6} & 61.9 & 40.3 \\
\midrule
\multirow{1}{1.2cm}[8pt]{\raggedright\scriptsize OpenX +\\Web Co-train} & 
\rule[-10pt]{0pt}{24pt} OpenPI0.5 & \textbf{98.4} & 88.3 & 79.0 & 62.4 & \textbf{99.4} & \textbf{97.1} & \textbf{88.4} & \textbf{76.4} & 97.2 & 87.2 & 82.5 & 64.2 & 92.0 & 76.1 & \textbf{65.6} & \textbf{47.7} \\
\midrule
\multirow{2}{1.2cm}{\raggedright\scriptsize VLM\\Direct FT} & VLA-Adapter-Pro & 96.0 & \underline{93.7} & 83.3 & 58.5 & 96.8 & 71.0 & 44.1 & 29.3 & \underline{97.4} & 79.5 & 64.7 & 47.3 & \underline{94.4} & 63.5 & 41.0 & 26.2 \\
 & StableVLA & \underline{96.2} & \textbf{94.3} & \textbf{92.1} & \textbf{82.0} & \underline{98.8} & \underline{92.4} & \underline{83.6} & \underline{70.2} & \textbf{98.0} & \underline{93.4} & \textbf{85.0} & \textbf{71.9} & 93.6 & \underline{76.3} & \underline{62.4} & \underline{45.3} \\
\bottomrule
\end{tabular}
\end{table}
